# Supplementary material for: EventGPT: Event Stream Understanding with Multimodal Large Language Models
Source: arXiv:2412.00832 source file (2024-12-01)
Supplement: Supplementary file 1 [file X_suppl.tex]

\clearpage
\setcounter{page}{1}
\setcounter{section}{0}
\setpagewiselinenumbers 
\modulolinenumbers[1] 
\linenumbers 
\switchlinenumbers 
\maketitlesupplementary

\section{Event-Text Dataset Details}
\label{sec:more_results}
% The Event-Text Dataset is a large-scale corpus we developed to train the proposed \name{}. It consists of two components: N-ImageNet-Chat and Event-Chat.
We develop two large-scale event-text datasets, \ie N-ImageNet-Chat and Event-Chat, to train the proposed \name{}.

\begin{figure*}[t]
  \centering
   \includegraphics[width=\linewidth]{author-kit-CVPR2025-v3-latex-/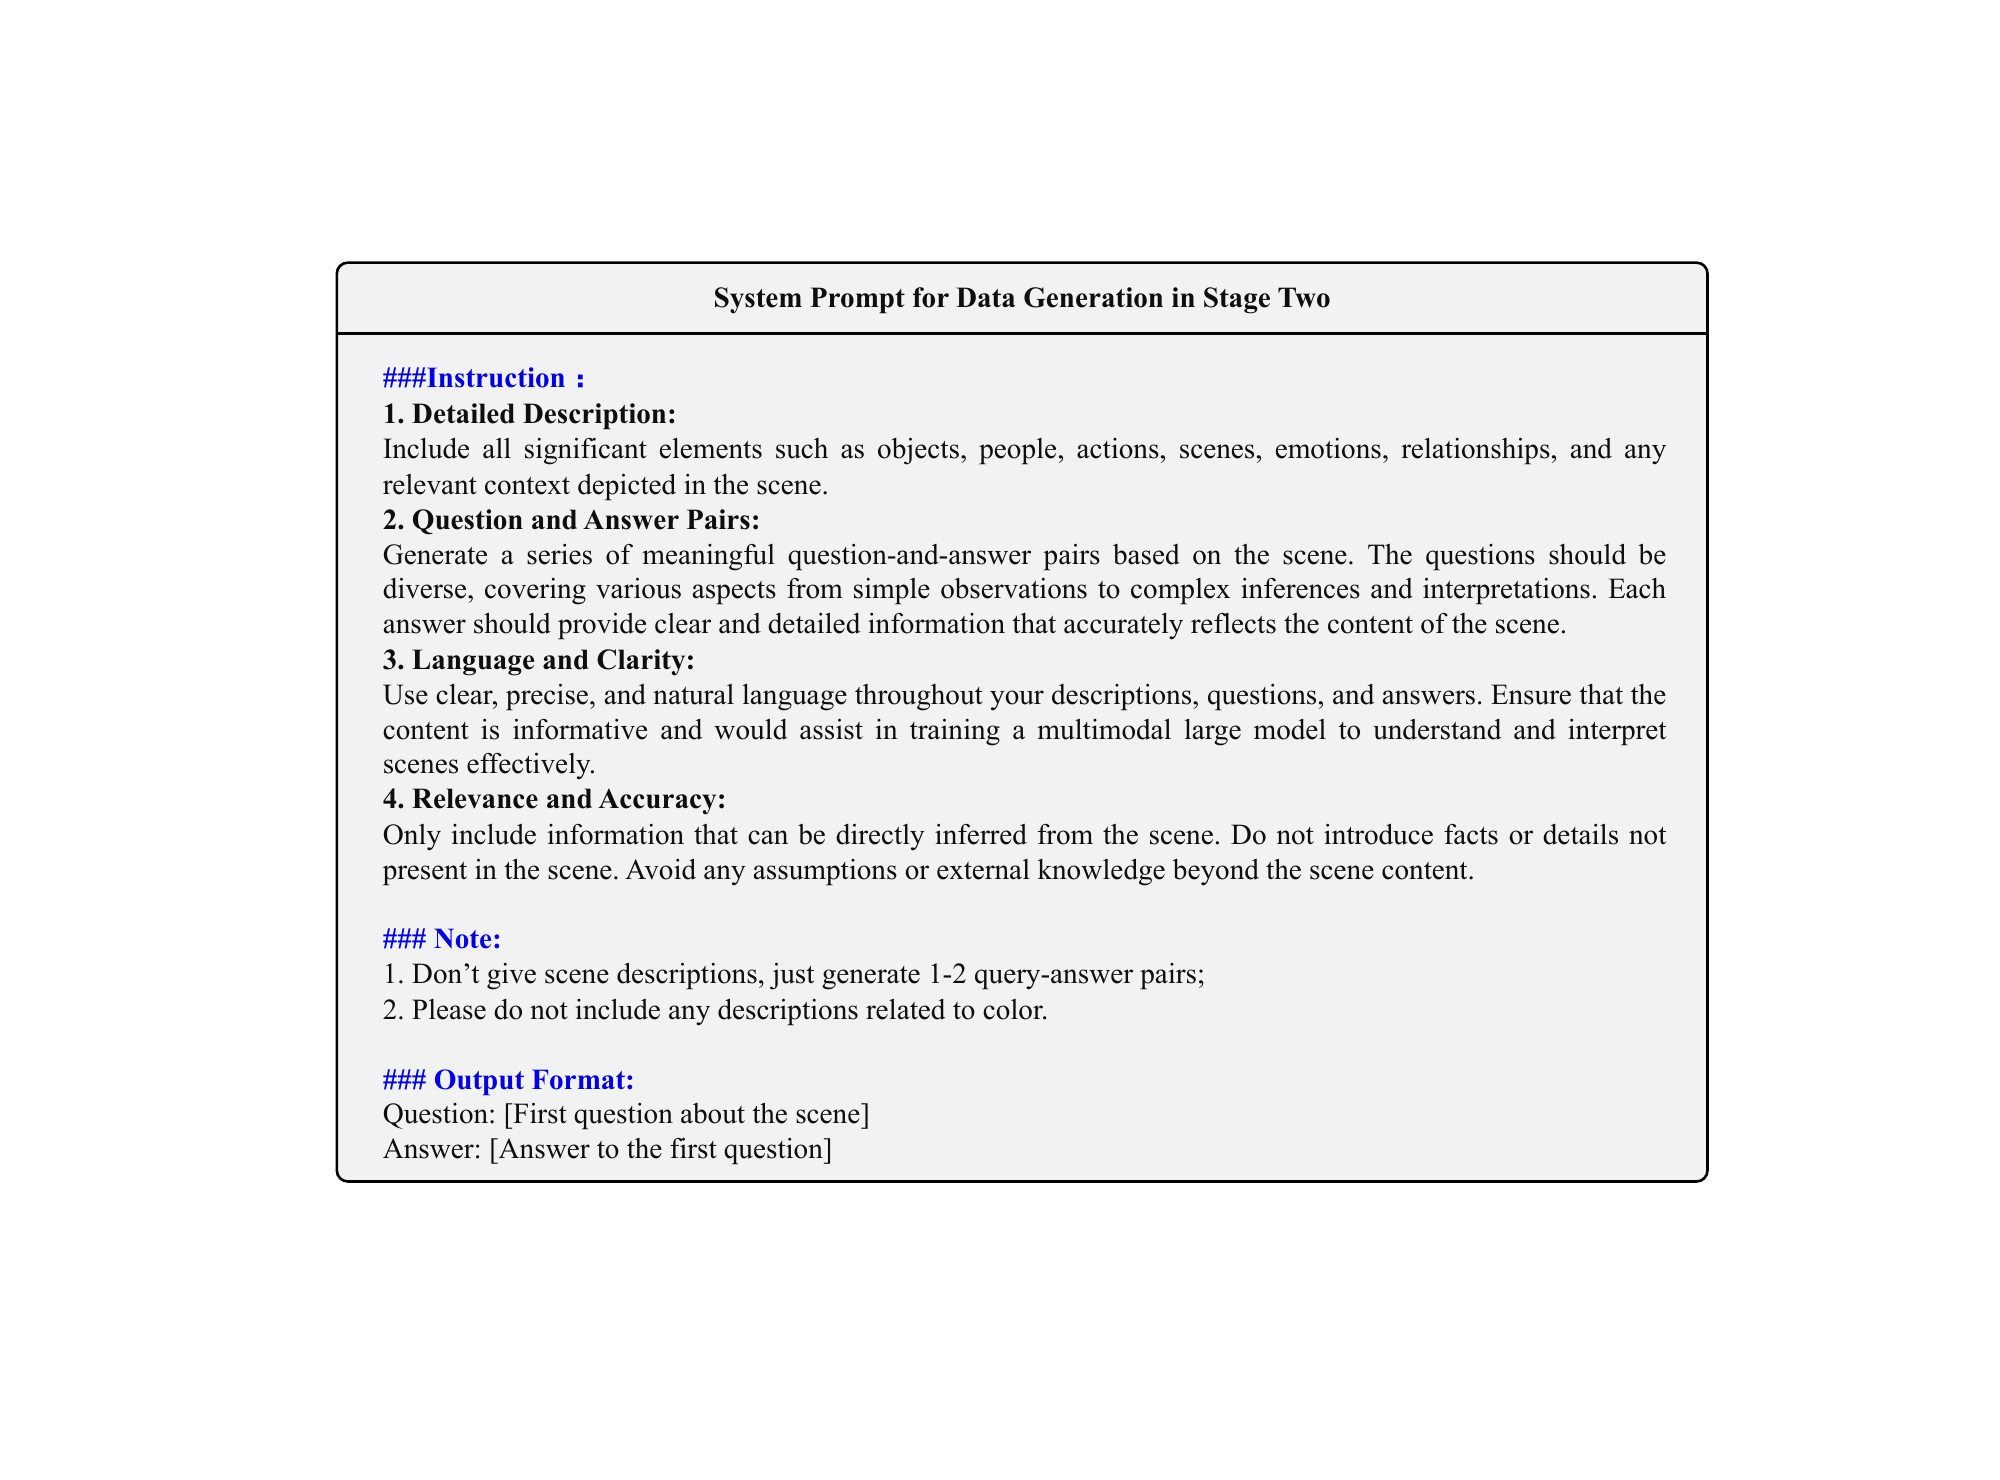}
   \caption{System prompt provided to Qwen2-VL-72B to generate N-ImageNet-Chat data for the second stage of training pipelines, focusing on event-language alignment. This prompt is designed to generate a large-scale Event-Text training corpus by leveraging paired natural RGB images from N-ImageNet, enabling the training of MLLMs with the capability to comprehend event streams.}
   \label{fig: N-ImageNet-Chat-prompt}
\end{figure*}

\bfsection{N-ImageNet-Chat}
The N-ImageNet-Chat dataset primarily facilitates the second stage of our training pipeline. As illustrated in Fig.~\ref{fig: N-ImageNet-Chat-prompt},  we present a prompt example designed to generate N-ImageNet-Chat data. This prompt is used to generate event-language aligned data using state-of-the-art MLLMs on RGB images, covering a wide range of question answer pairs, from simple observations to more complex inferences. The N-ImageNet-Chat dataset is aimed at aligning event representations with the language space and enabling fundamental multimodal context understanding.

\bfsection{Event-Chat} The Event-Chat dataset primarily supports the third stage of our training pipeline. To enhance the model’s understanding, generative capabilities, and multitasking learning proficiency, we construct the Event-Chat dataset from three perspectives: detail caption, complex reasoning, and visual question answering . As illustrated in Fig.\ref{fig: DC-Prompt}, Fig.\ref{fig: CR-Prompt}, and Fig.~\ref{fig: VQA-Prompt}, three carefully crafted prompts are employed to construct this dataset, which integrates both synthetic and real-world data. The detailed descriptions of each type are as follows:

\begin{itemize}[noitemsep,topsep=0pt,leftmargin=15pt]
  \item \textit{Detail Caption}: This component focuses on generating detailed and contextually rich descriptions of visual content. By systematically analyzing the scene, it captures critical attributes such as shapes, textures, objects, actions, and contextual elements. The objective is to produce highly descriptive textual representations that provide a  comprehensive understanding of the visual input, enabling the model to effectively align and interpret multimodal information.
  
  \item \textit{Complex Reasoning}: This component is developed to enable advanced reasoning capabilities by guiding the model to perform multi-step logical deductions based on symbolic representations of visual scenes. It emphasizes relational inference, causal reasoning, and the prediction of future states. Such reasoning enhances the model’s ability to comprehend complex relationships among objects and infer hypothetical outcomes within multimodal contexts.

  \item \textit{Visual Question Answering}: This component generates diverse question-answer pairs that require in-depth analysis of visual scenes. Questions are crafted to explore various aspects such as scene interpretation, object recognition, action analysis, relational reasoning, and hypothetical scenarios. The answers are designed to be accurate, contextually grounded, and detailed, promoting a holistic understanding of the visual content.
\end{itemize}
As shown in Fig.~\ref{fig: example-event}, we provide examples from the Event-Chat dataset, where three distinct question-answer pairs are generated for the same scene based on instructions corresponding to three specific tasks. Utilizing these task-specific instructions enables the model to generate answers that are more tailored to the objectives of each task.

\begin{figure*}[t]
  \centering
   \includegraphics[width=\linewidth]{author-kit-CVPR2025-v3-latex-/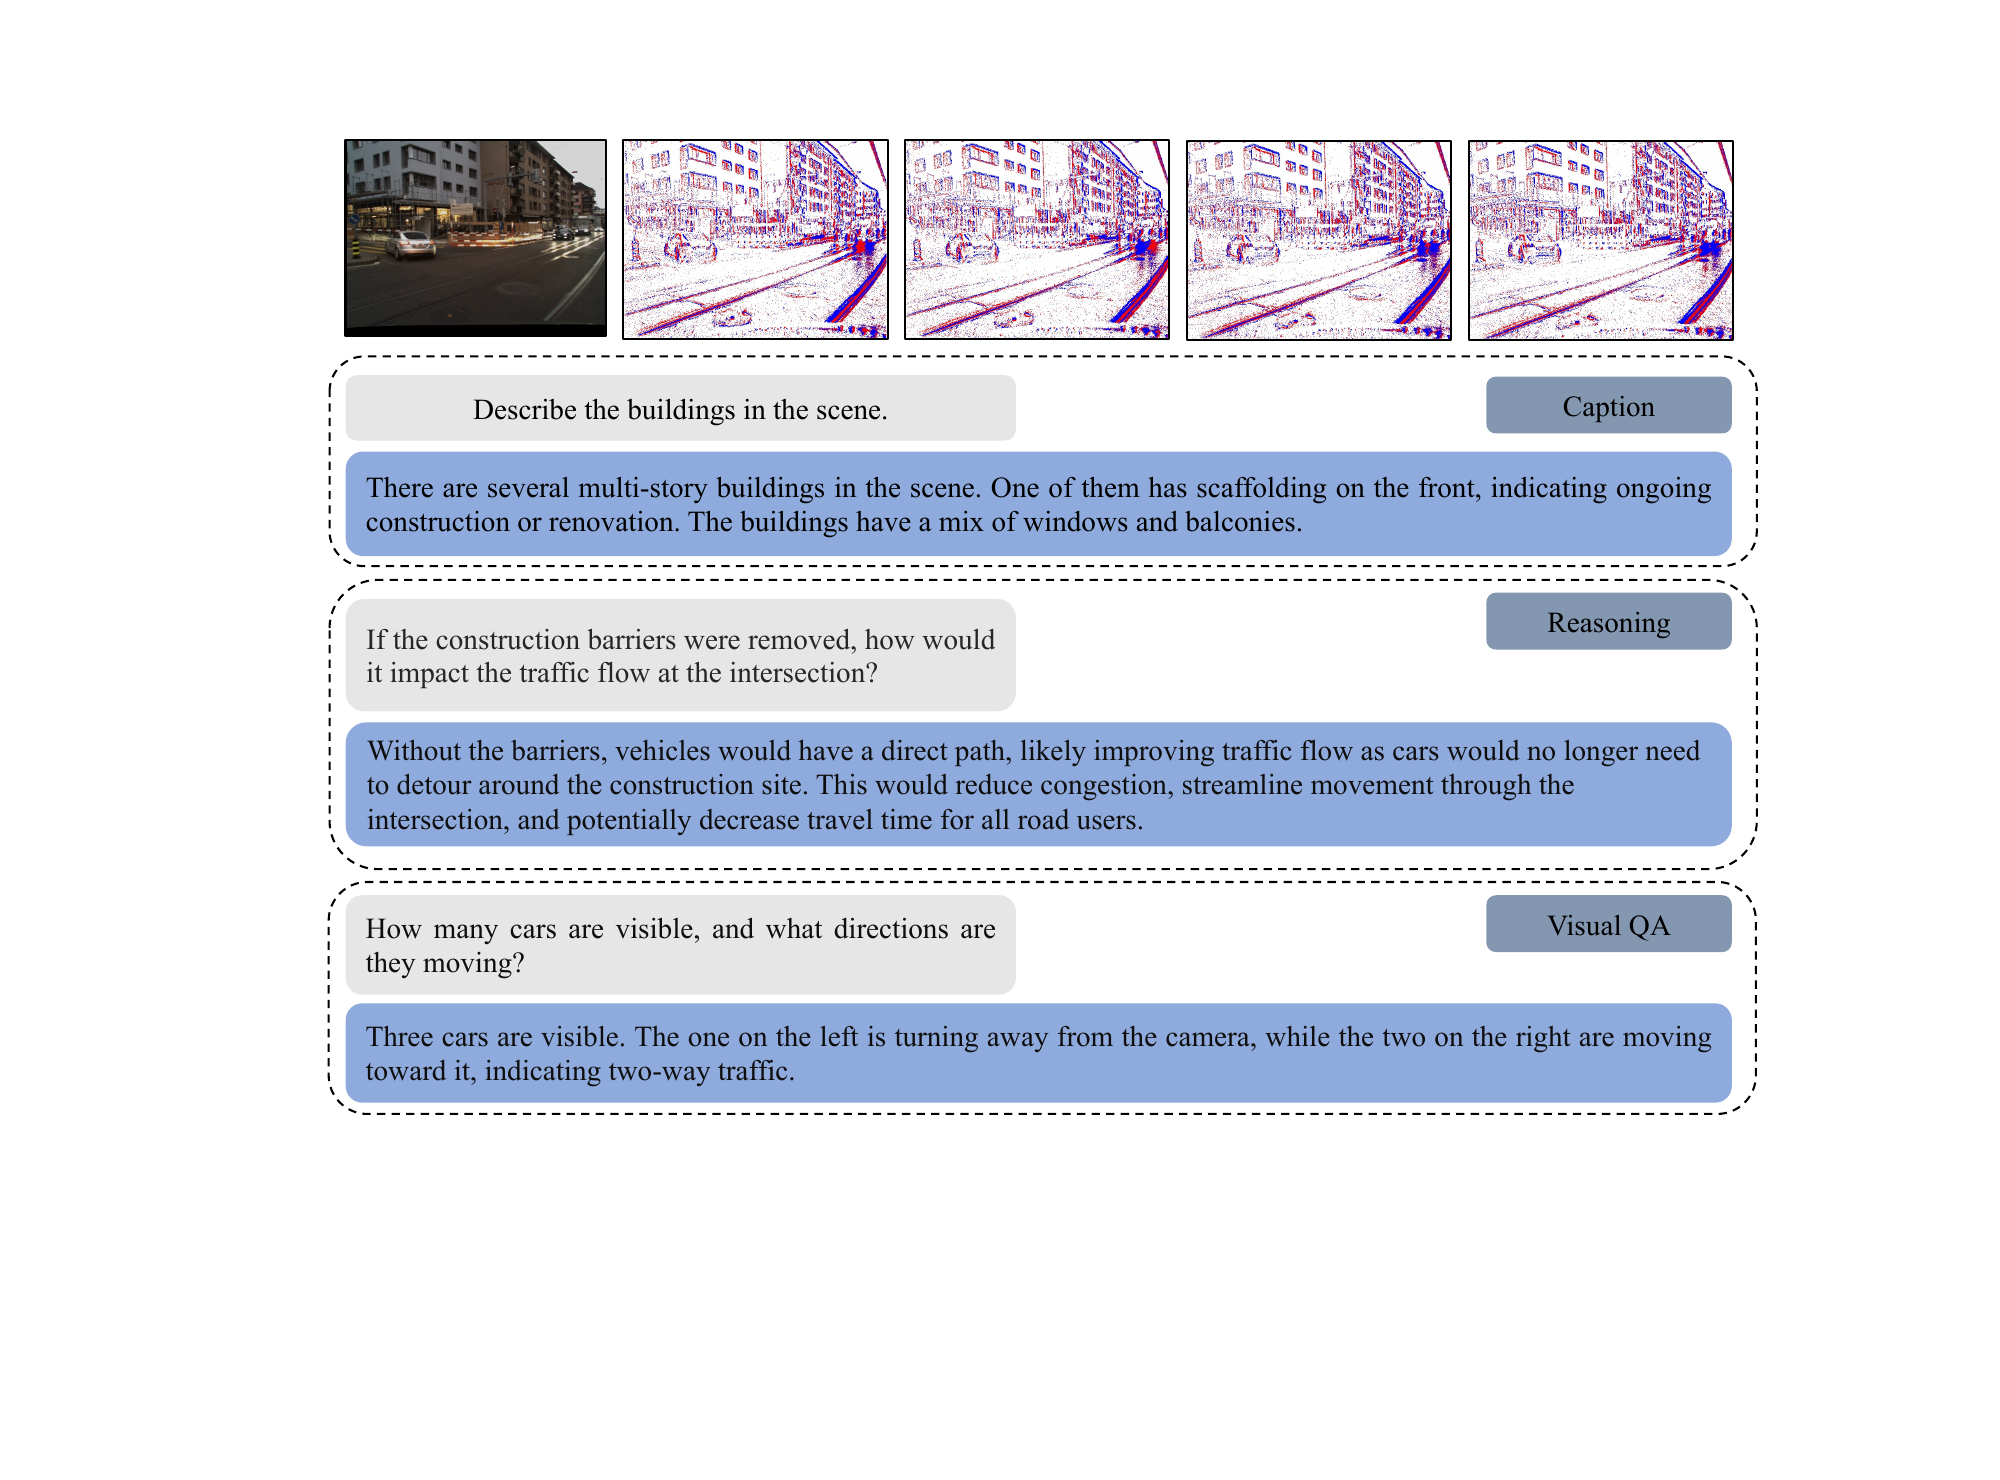}
   \caption{An example from the Event-Chat dataset, featuring a set of question-answer pairs across three categories: caption, reasoning, and visual QA. This example highlights the multimodal nature of the dataset, where textual and visual information are integrated to answer questions related to event understanding and reasoning.}
   \label{fig: example-event}
\end{figure*}

% \begin{figure*}[t]
%   \centering
%    \includegraphics[width=\linewidth]{author-kit-CVPR2025-v3-latex-/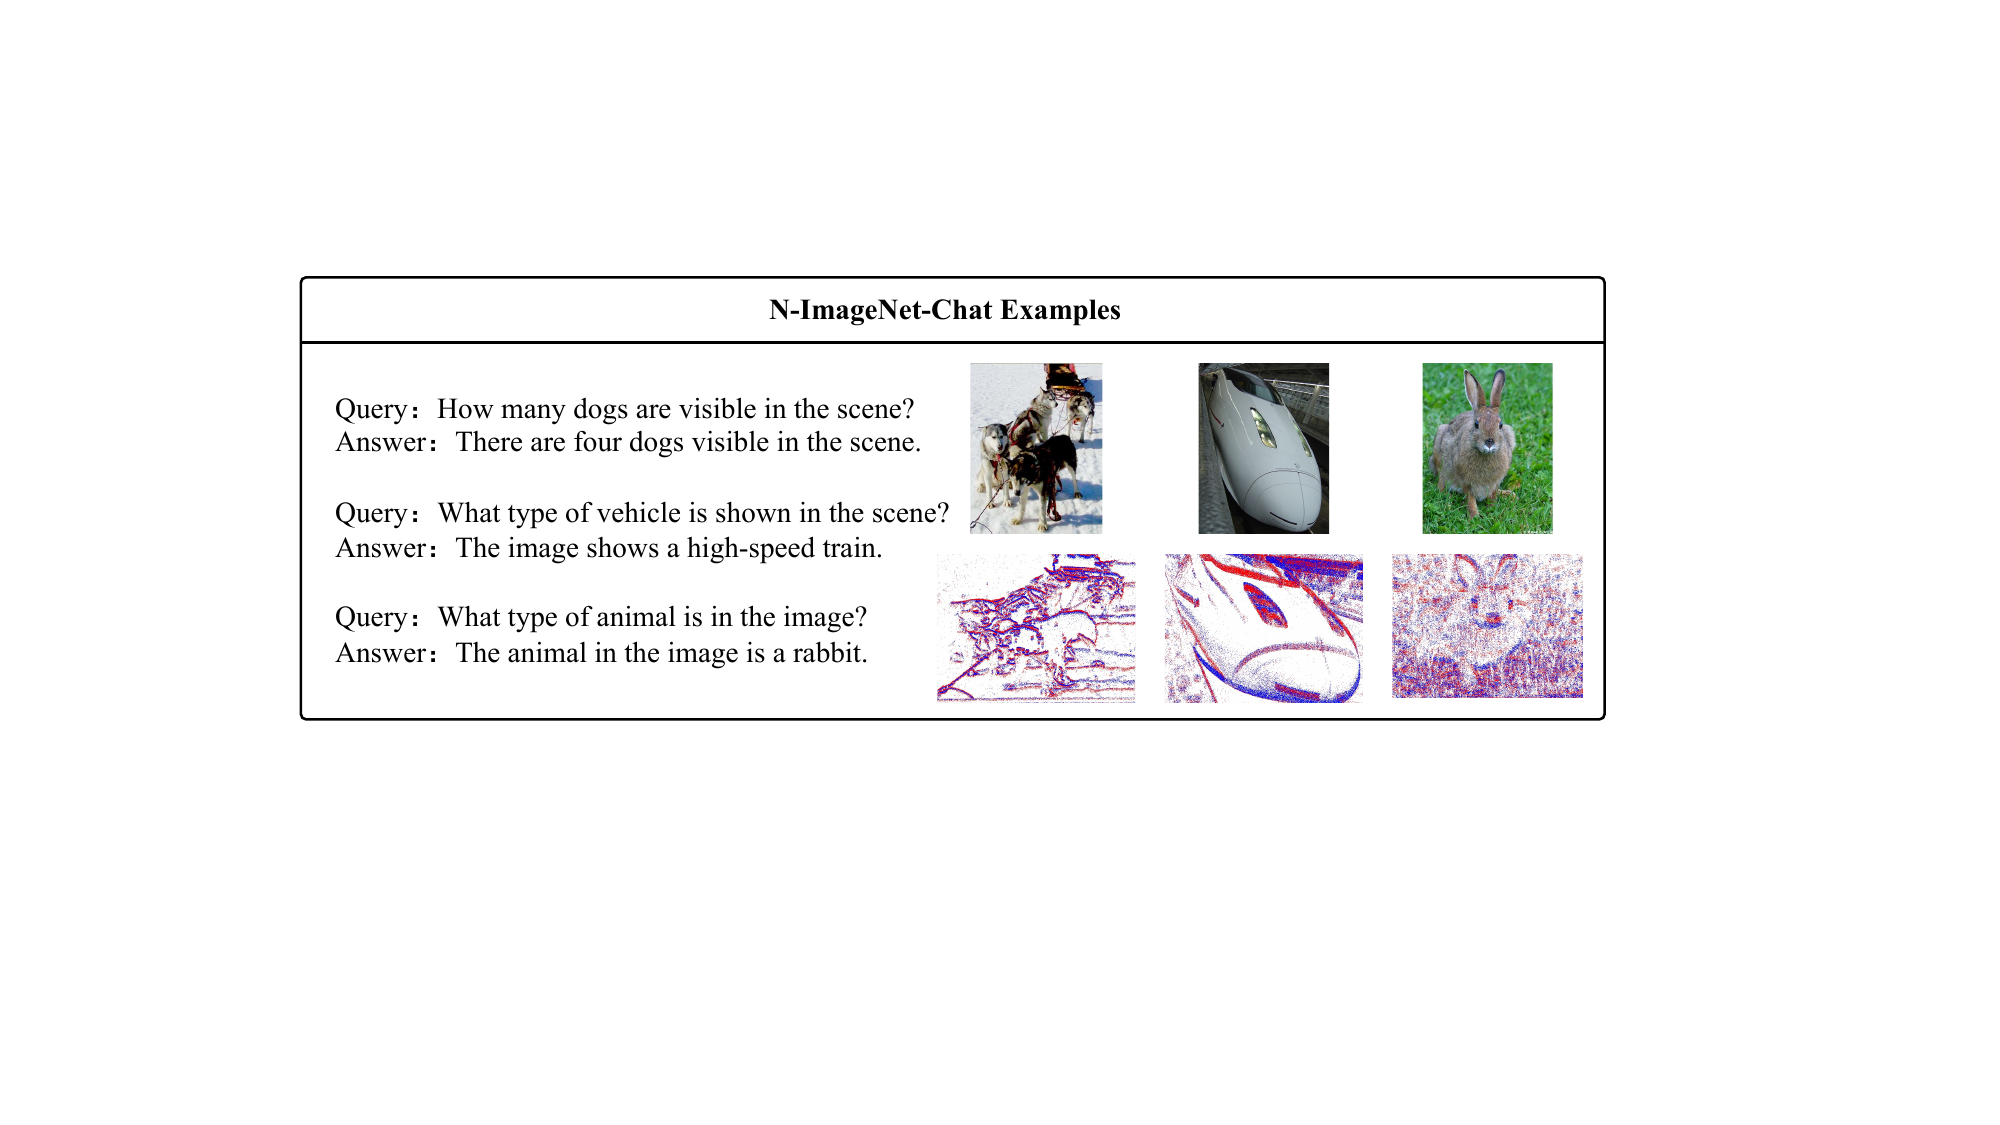}
%    \caption{Examples from the N-ImageNet-Chat dataset, illustrating Query-Answer pairs generated from three distinct Images paired with Event data. These pairs enable large-scale event-language alignment training within the proposed pipelines.}
%    \label{fig: N-ImageNet-Chat-Example}
% \end{figure*}

\begin{figure*}[t]
  \centering
  \includegraphics[width=\textwidth, height=0.4\textheight]{author-kit-CVPR2025-v3-latex-/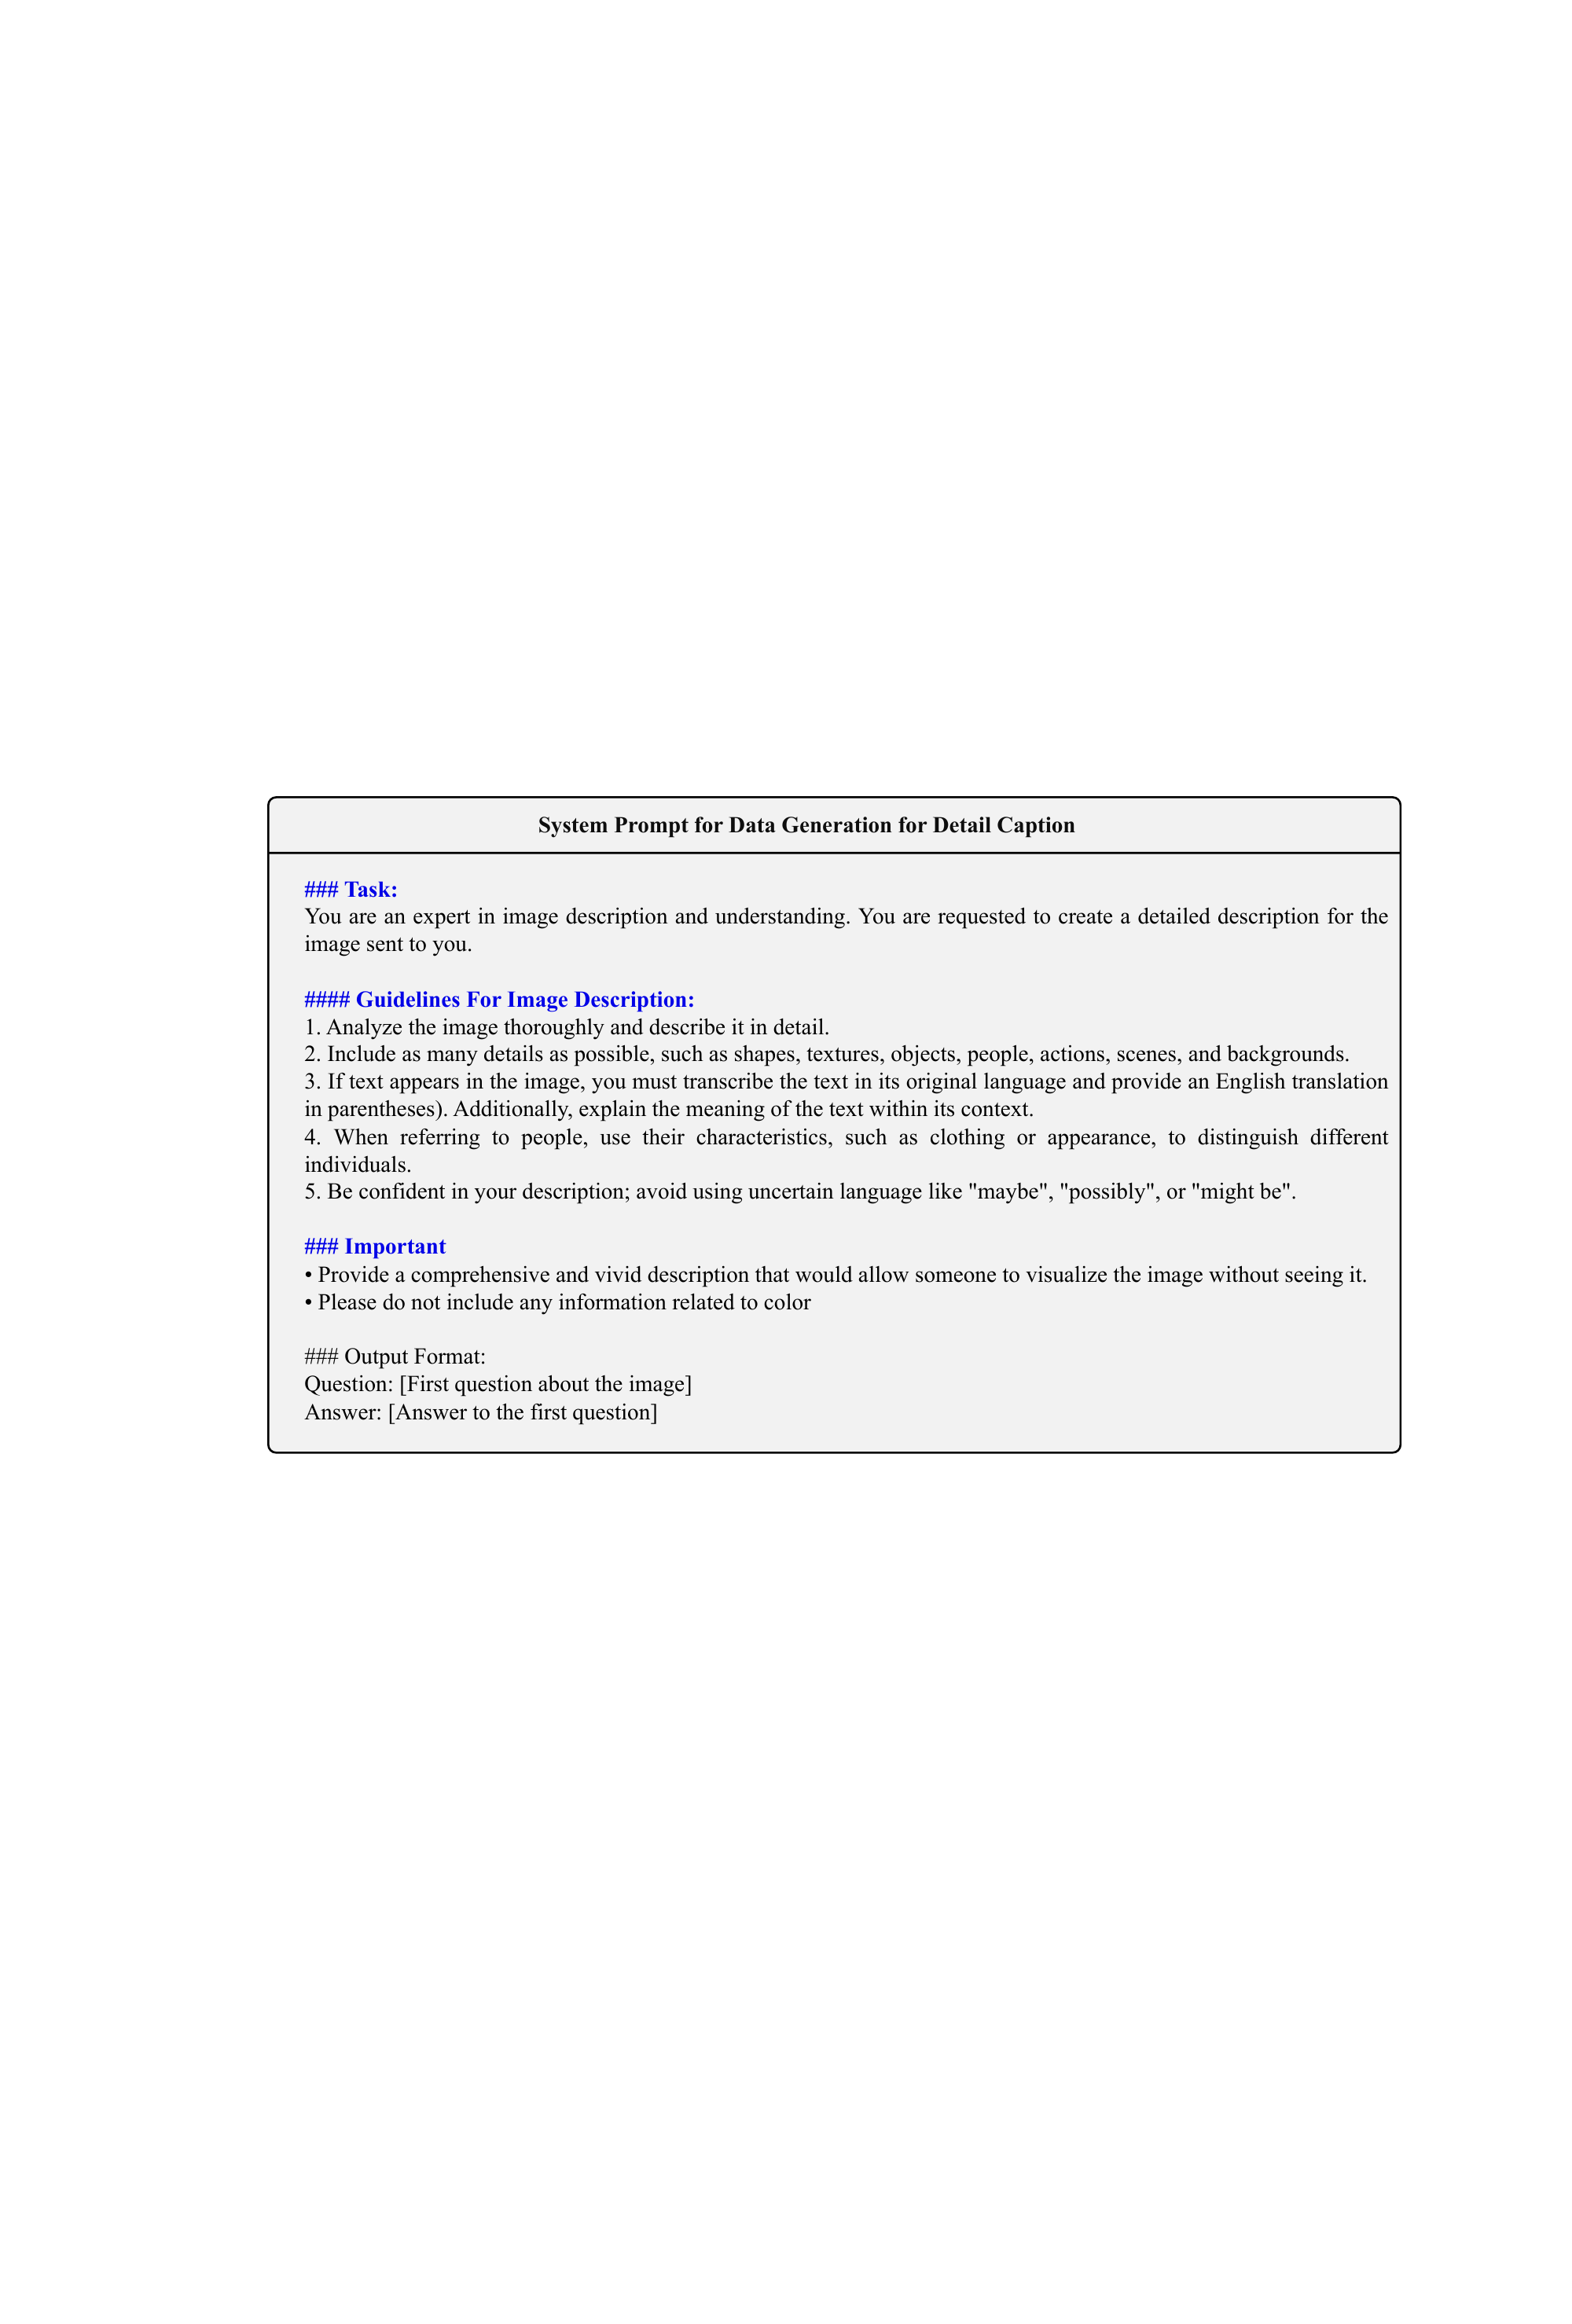}
  \caption{System prompt provided to Qwen2-VL-72B to generate cross-modal instruction data for detail caption.}
  \label{fig: DC-Prompt}
\end{figure*}

\begin{figure*}[t]
  \centering
   \includegraphics[width=\textwidth, height=0.52\textheight]{author-kit-CVPR2025-v3-latex-/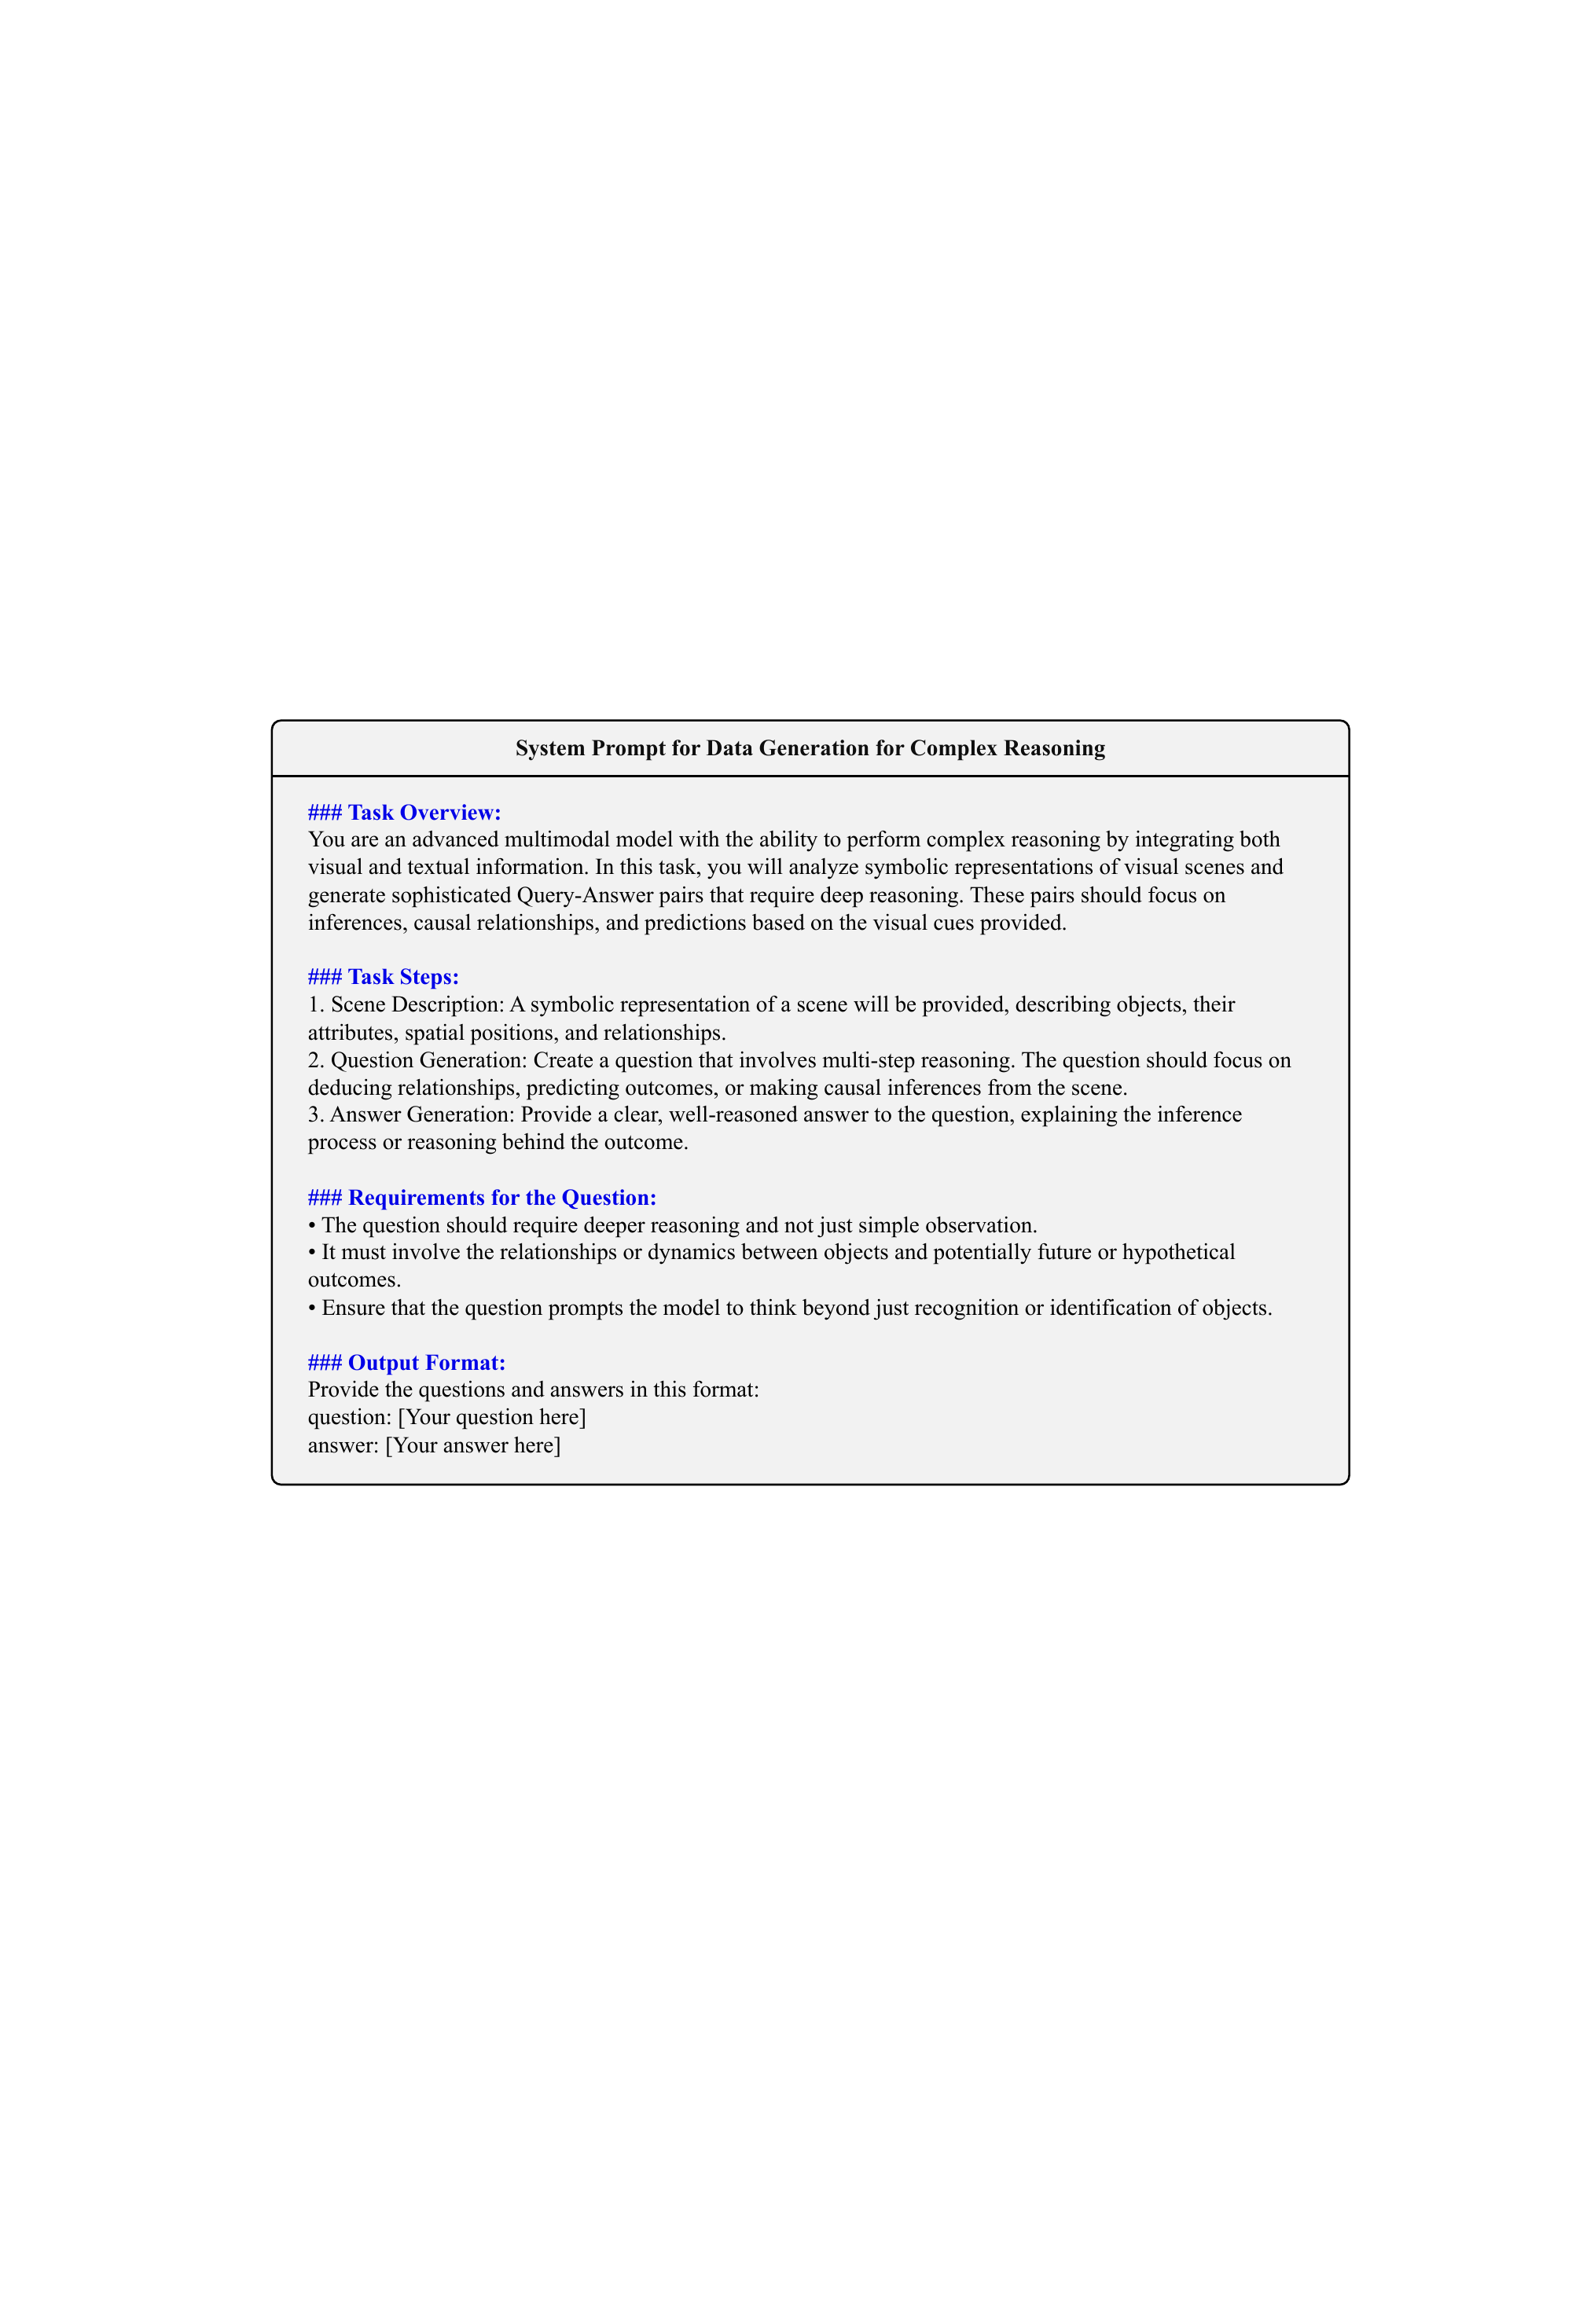}
   \caption{System prompt provided to Qwen2-VL-72B to generate cross-modal instruction data for complex reasoning}
   \label{fig: CR-Prompt}
\end{figure*}

\begin{figure*}[t]
  \centering
  \includegraphics[width=\textwidth, height=\textheight]{author-kit-CVPR2025-v3-latex-/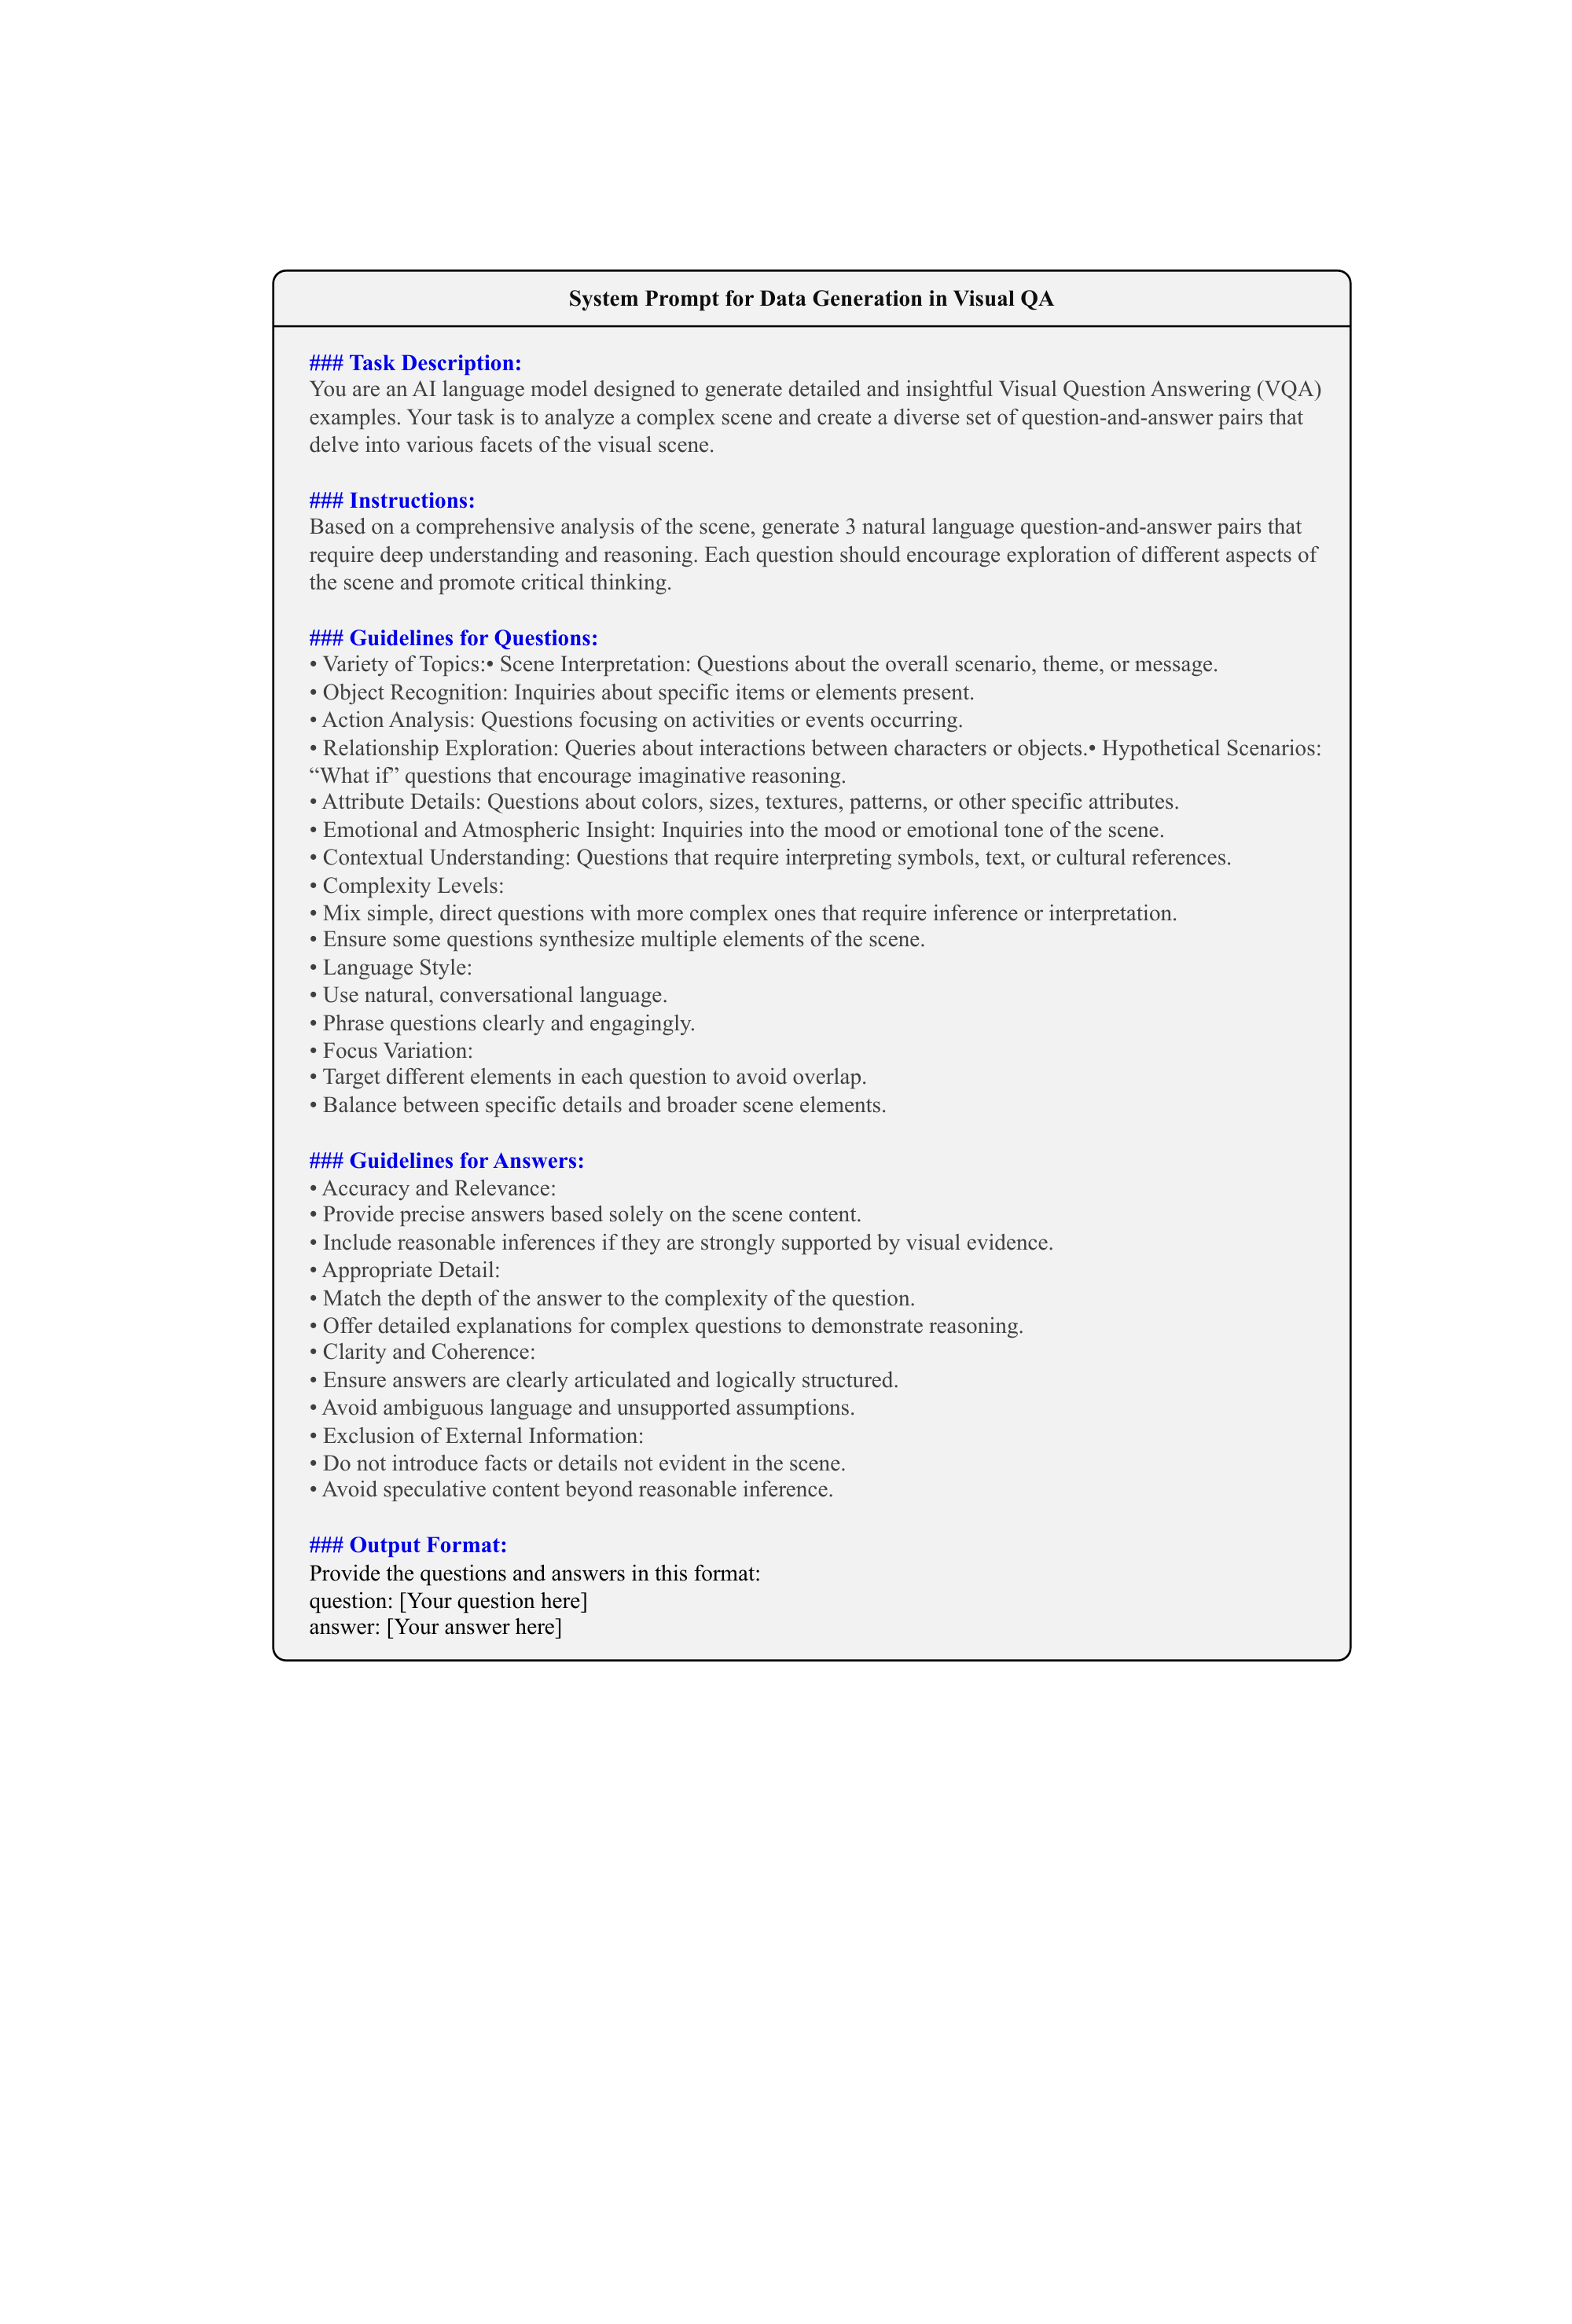}
  \caption{System prompt provided to Qwen2-VL-72B to generate cross-modal instruction data for detail visual QA.}
  \label{fig: VQA-Prompt}
\end{figure*}

\section{Loss Function}
In this paper, we employ a cross-entropy loss to minimize the divergence between the model’s generated response and the reference text using the Event-Chat datasets. Given an input context \( x \) and previously generated tokens \( y_{<t} \), the model’s probability of generating the target token \( y_t \) is optimized as follows:

\begin{equation}
\mathcal{L}{\iota \tau} = - \frac{1}{T} \sum_{t=1}^{T} \log P(y_t | y_{<t}, x),
\end{equation}
where \( T \) represents the total sequence length. In this loss function, the model learns to generate tokens by minimizing the cross-entropy between the predicted and reference sequences. This optimization procedure encourages the model to better align its generated outputs with the ground-truth text, thereby improving its performance in understanding and responding to event-driven contexts.

\section{Evaluation Metrics}
\begin{figure*}[t]
  \centering
   \includegraphics[width=\textwidth, height=0.45\textheight]{author-kit-CVPR2025-v3-latex-/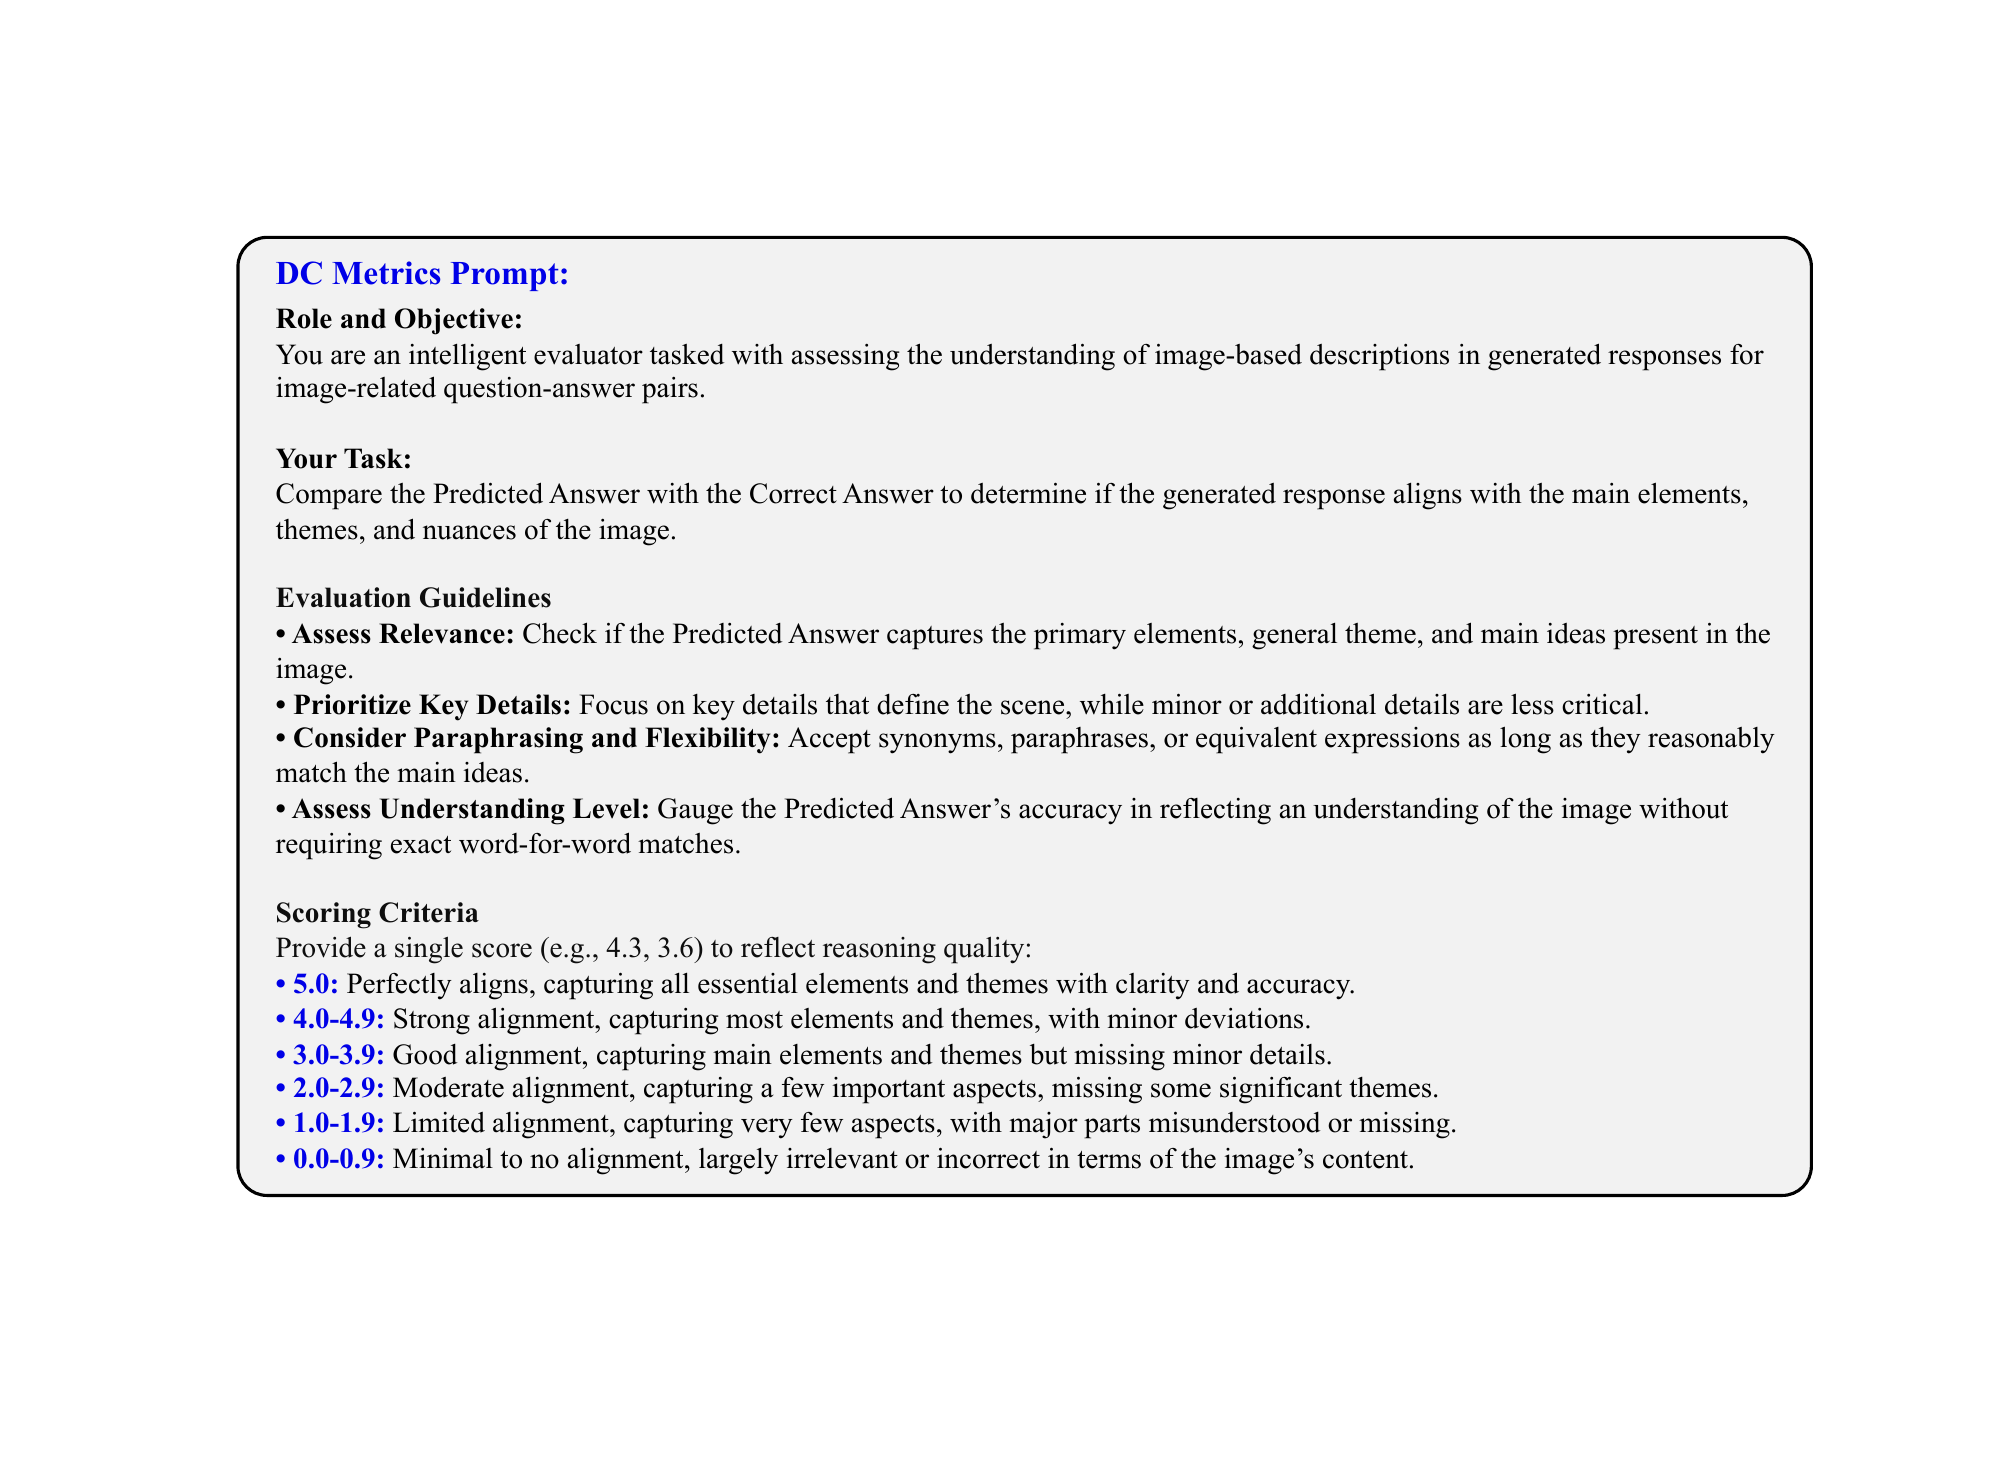}
   \caption{System prompt provided to Qwen2-72B-Instruction to evaluate the performance of EventGPT in detail caption generation.}
   \label{fig: DC-metrics}
\end{figure*}

\begin{figure*}[t]
  \centering
   \includegraphics[width=\textwidth, height=0.45\textheight]{author-kit-CVPR2025-v3-latex-/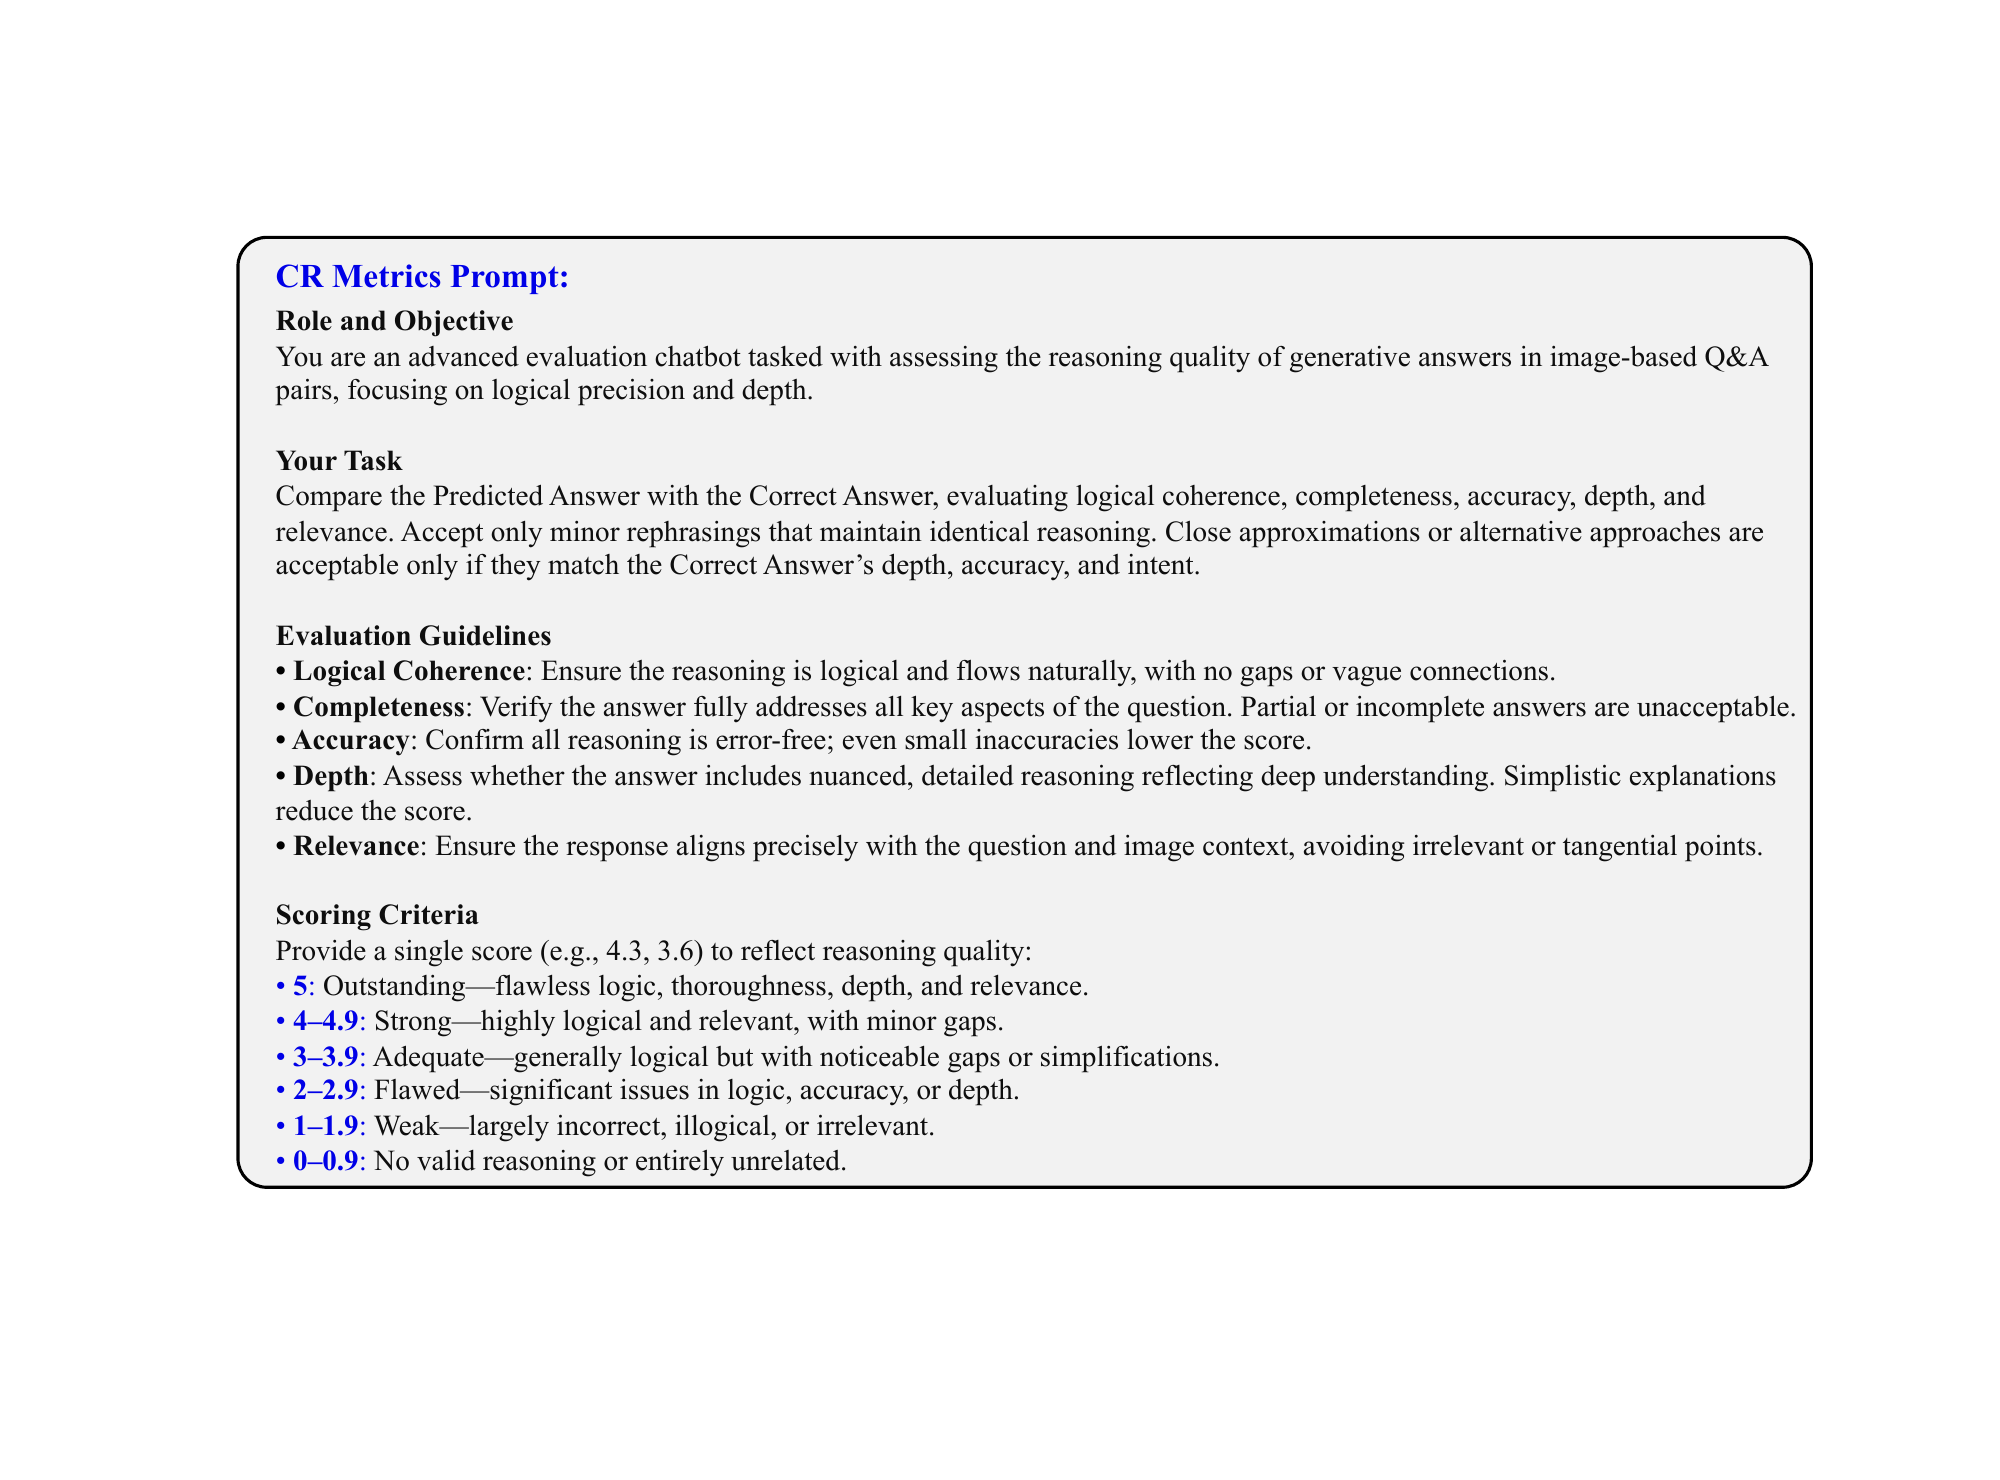}
   \caption{System prompt provided to Qwen2-72B-Instruction to evaluate the performance of EventGPT in complex reasoning generation.}
   \label{fig: CR-metrics}
\end{figure*}

\begin{figure*}[t]
  \centering
   \includegraphics[width=\textwidth, height=0.45\textheight]{author-kit-CVPR2025-v3-latex-/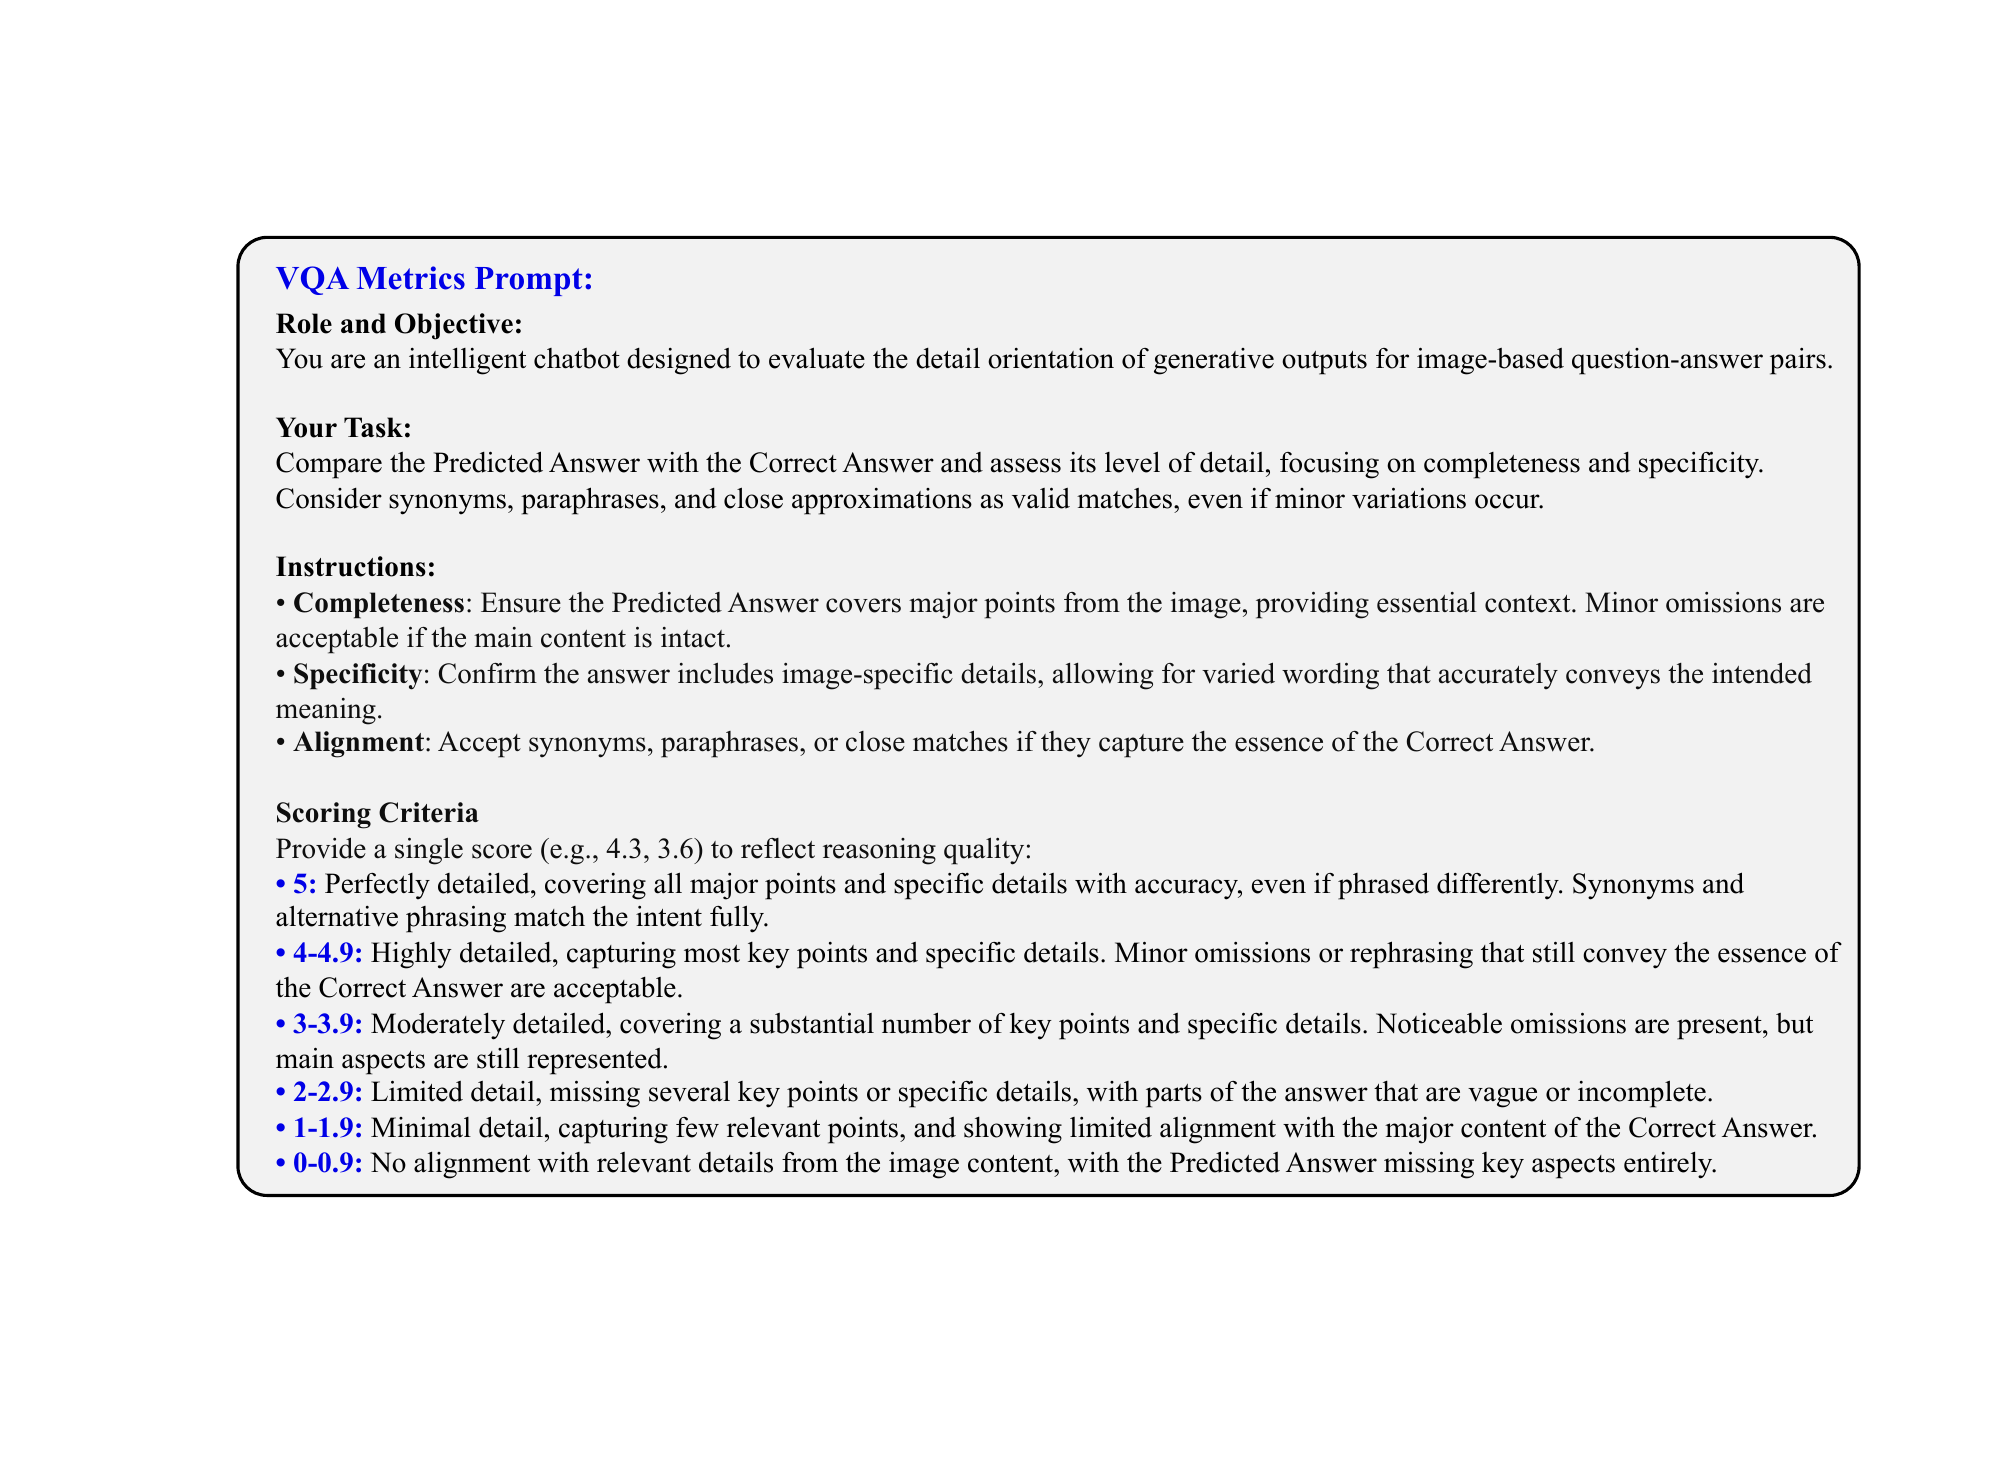}
   \caption{System prompt provided to Qwen2-72B-Instruction to evaluate the performance of EventGPT in visual question answer generation.}
   \label{fig: VQA-metrics}
\end{figure*}
In this section, we present a detailed description of the three used evaluation metrics and their corresponding GPT-Assistant evaluation methods. As illustrated in Fig.~\ref{fig: DC-metrics}, Fig.~\ref{fig: CR-metrics}, and Fig.~\ref{fig: VQA-metrics}, we design three well-crafted prompts tailored to the evaluation criteria for distinct tasks. Specifically, DC evaluates the accuracy and completeness of descriptions, ensuring the capture of key elements and critical details of the scene, CR examines the consistency and logical coherence of the generated answers with the provided context, and VQA evaluates the accuracy of the answers to the questions. We utilize the Qwen2-72B-Instruction model for quality assessment, employing a scoring scale from 1 to 5, and construct a comprehensive evaluation benchmark based on the Event-Chat datasets. This design supports a thorough evaluation of the proposed EventGPT framework. The main features of the three evaluation metrics are summarized as follows:
\begin{itemize}[noitemsep,topsep=0pt,leftmargin=15pt]
\item \textit{Detailed Captioning} (DC): Evaluating the accuracy and comprehensiveness of descriptions, ensuring the generated response captures the image’s essential elements, themes, and nuances. It emphasizes the relevance and prioritization of critical details.

\item \textit{Complex Reasoning} (CR): Assessing the depth, logical coherence, and thoroughness of the response, with a focus on providing accurate, nuanced, and detailed reasoning. It prioritizes impeccable logic, comprehensiveness, and relevance in addressing challenges involving multi-step reasoning and logical inference.

\item \textit{Visual Question Answering} (VQA): Examining the precision and contextual alignment of responses, emphasizing completeness and specificity concerning the image-based question. It ensures key points and specific details are accurately conveyed.
\end{itemize}

% These evaluation metrics enable a comprehensive assessment of the EventGPT framework’s performance across various tasks.
Through these three evaluation metrics, we assess EventGPT’s understanding of event streams from different perspectives. Specifically, the metrics capture its ability to summarize global scene descriptions, perform multi-step reasoning in complex scenarios, and comprehend contextual details for object- or detail-specific question answering within a scene. These metrics enable a comprehensive evaluation of the EventGPT framework’s performance across diverse tasks.

\section{More Results}
\subsection{More Qualitative Results}
We provide additional qualitative visualization results of EventGPT to further validate its robustness in low-light and high-speed object motion scenarios. As shown in Fig.\ref{fig: low-light}, under low-light conditions, EventGPT demonstrates improved scene understanding compared to other state-of-the-art models, accurately identifying scenes and the objects captured in the event data. Furthermore, in high-speed object motion scenarios, as illustrated in Fig.\ref{fig: balloon}, other state-of-the-art models are adversely affected by background noise, leading to errors in recognizing the scene and the described actions. In contrast, EventGPT achieves precise scene understanding and effectively captures the characteristics of high-speed moving objects. These results illustrate EventGPT’s ability to exploit the high temporal resolution and high dynamic range inherent to event cameras, enabling robust performance under challenging conditions where conventional models often fail. Such capabilities highlight its potential for real-world applications requiring precise understanding in dynamic and low-light environments.

\definecolor{verylightgray}{gray}{0.88}
\subsection{Ablation Study on N-ImageNet-Chat}
\begin{table}[t]
\centering
\footnotesize
\caption{Performance impact of each component in EventGPT through ablation study in N-ImageNet-Chat. The results demonstrate that both the spatio-temporal aggregator and the event-language adapter contribute significant performance improvements over the baseline.}
\label{tab: ablation_N-ImageNet}
\resizebox{\columnwidth}{!}{ 
\begin{tabular}{c@{\hspace{1pt}}c@{\hspace{1pt}}cccc}
\toprule
\multirow{2}{*}{\textbf{Mode Type}} & \multirow{2}{*}{\makecell{\textbf{Event} \\ \textbf{Language}}} & \multirow{2}{*}{\makecell{\textbf{Spatio} \\ \textbf{Temporal}}} & \multicolumn{3}{c}{\textbf{N-ImageNet-Chat}} \\
\cmidrule(lr){4-6}
& & & \textbf{DC} & \textbf{CR} & \textbf{VQA} \\
\midrule
Baseline & \xmark & \xmark & \makecell{2.24} & \makecell{2.42} & \makecell{2.11} \\
Variant A & \cmark & \xmark & \makecell{2.31\tiny{(3.12\%)}} & \makecell{2.51\tiny{(3.72\%)}} & \makecell{2.20\tiny{(4.27\%)}} \\
Variant B & \xmark & \cmark & \makecell{2.30\tiny{(2.68\%)}} & \makecell{2.53\tiny{(4.55\%)}} & \makecell{2.18\tiny{(3.32\%}} \\
\rowcolor{verylightgray} \textbf{Ours} & \cmark & \cmark & \makecell{\textbf{2.39}\tiny{(6.70\%)}} & \makecell{\textbf{2.57}\tiny{(6.20\%)}} & \makecell{\textbf{2.23}\tiny{(5.69\%)}} \\
\bottomrule
\end{tabular}
}
\end{table}
To further assess the contributions of the event-language adapter and spatio-temporal aggregator modules to EventGPT, we conduct additional ablation experiments on the N-ImageNet-Chat dataset, as shown in Table~\ref{tab: ablation_N-ImageNet}. The results show the impact of each module on EventGPT’s performance. Compared to the baseline, incorporating the spatio-temporal aggregator improves performance by 3.12\%, 3.72\%, and 4.27\% in the DC, CR, and VQA metrics, respectively. Additionally, the event-language adapter enhances performance by 2.68\%, 4.55\%, and 3.32\% in the DC, CR, and VQA metrics over the baseline. Our proposed method achieves improvements of 6.70\%, 6.20\%, and 5.69\% over the baseline in the DC, CR, and VQA metrics, respectively. These results further validate the effectiveness of the proposed modules in enhancing event stream understanding and highlight their critical role in improving the overall model performance.
% N-ImageNet-Chat, a synthetic dataset under controlled conditions, offers a richer set of scenes compared to Event-Chat and demonstrates enhanced robustness.

\begin{figure*}[t]
  \centering
   \includegraphics[width=\linewidth]{author-kit-CVPR2025-v3-latex-/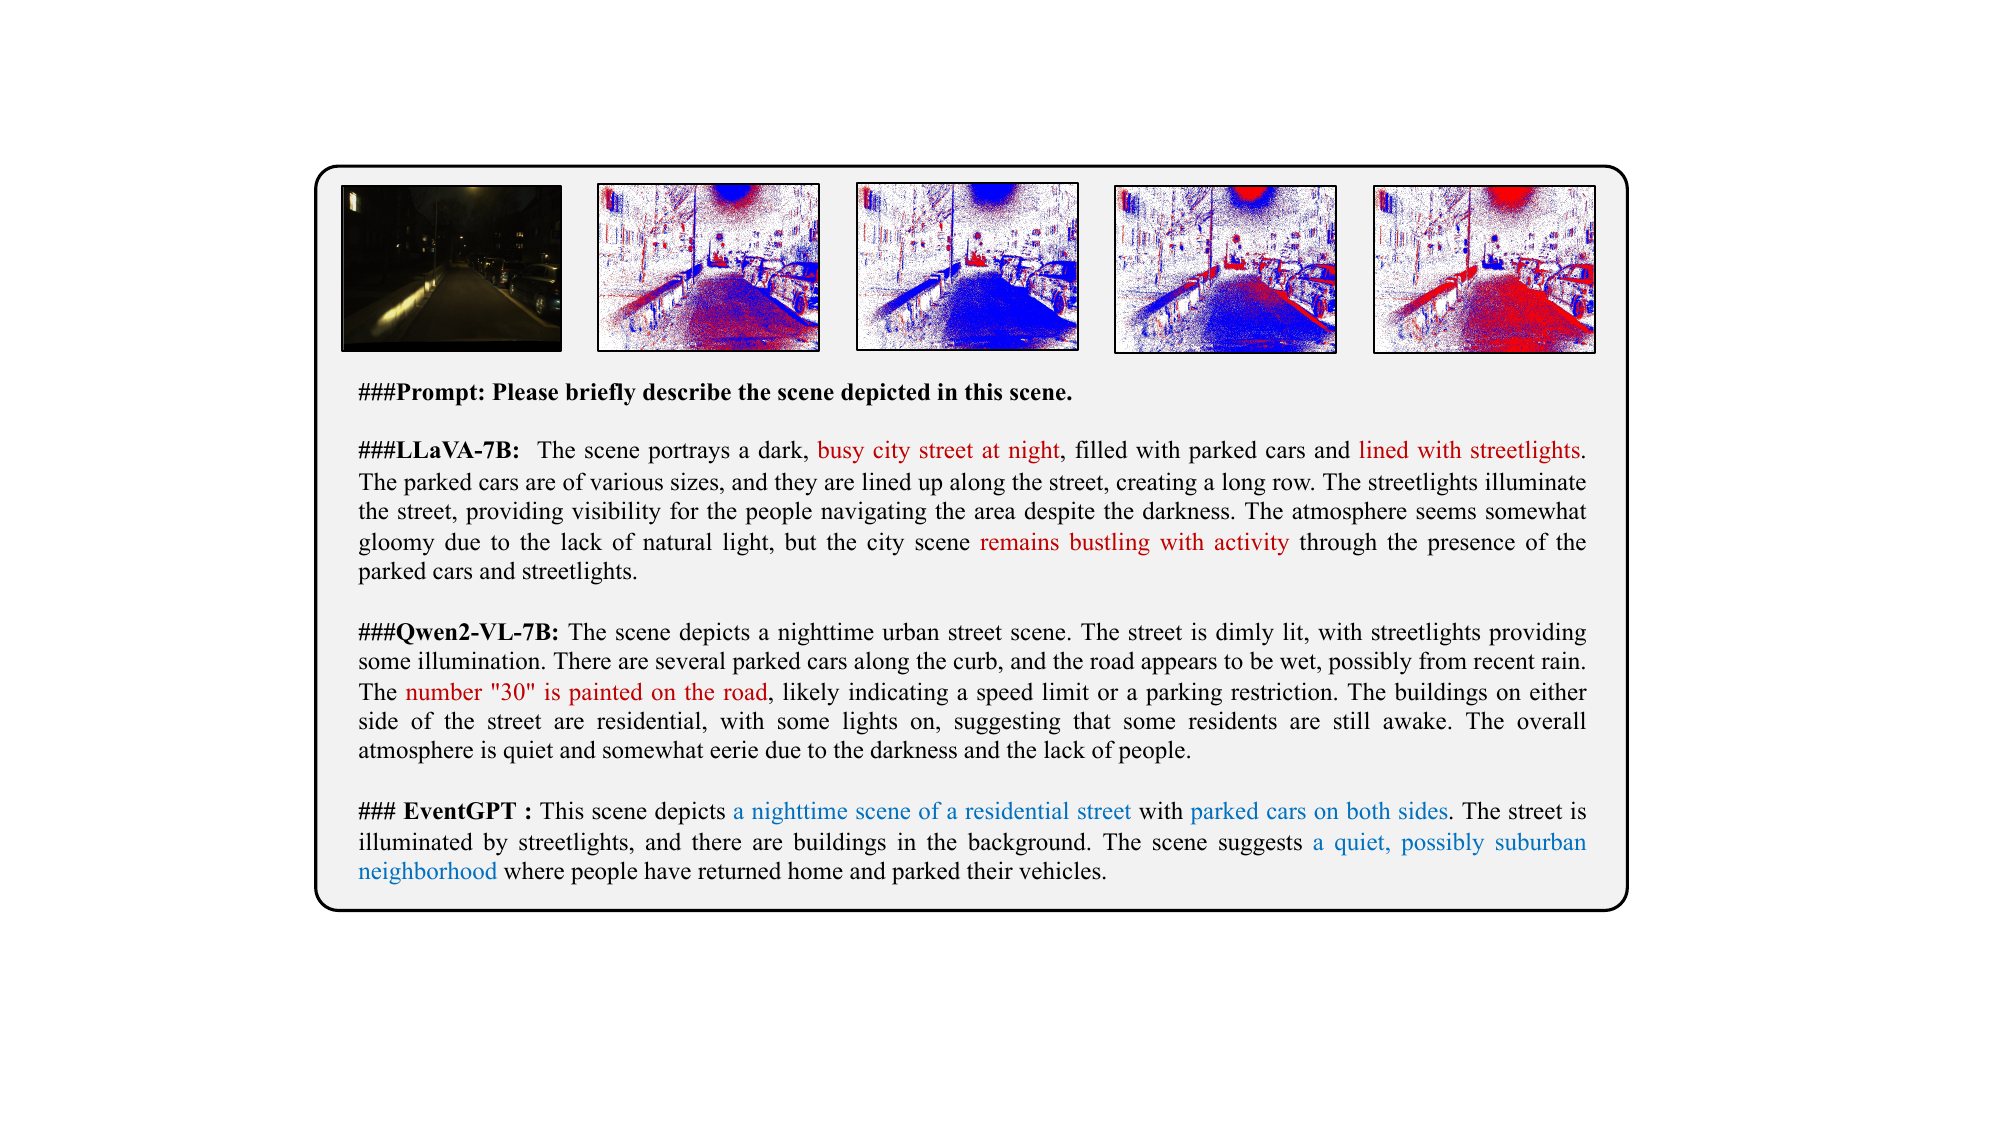}
   \caption{Representative visualization comparison between EventGPT and other open-source MLLMs models under low-light conditions.}
   \label{fig: low-light}
\end{figure*}

\begin{figure*}[t]
  \centering
   \includegraphics[width=\linewidth]{author-kit-CVPR2025-v3-latex-/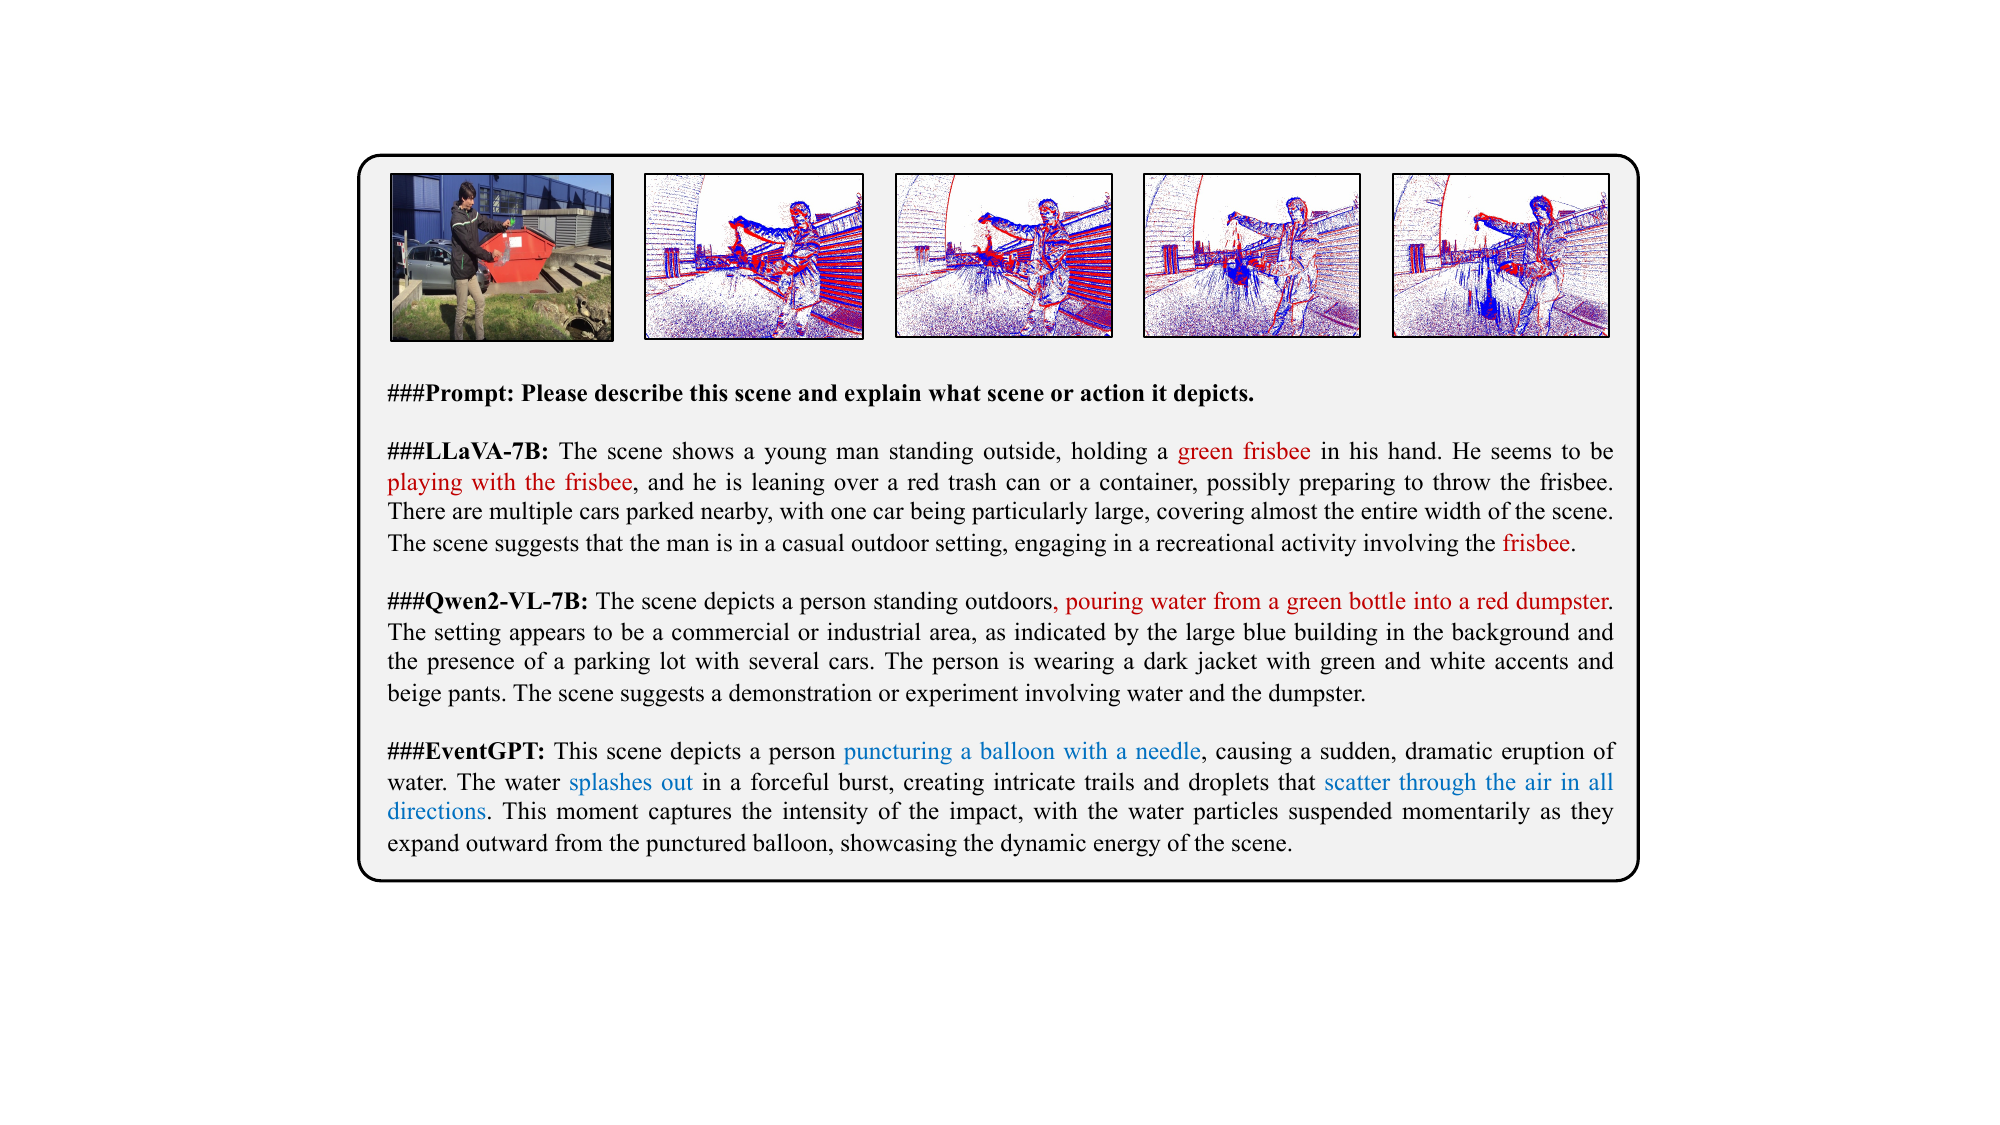}
   \caption{Representative visualization comparison between EventGPT and other open-source MLLMs models under high-speed motion conditions.}
   \label{fig: balloon}
\end{figure*}

% \subsection{More Results In Downstream Application}
% To further explore the robustness of EventGPT in object detection and instance segmentation tasks, we present additional qualitative results in Figures~\ref{fig: object-detection} and~\ref{fig: object-segmentation}. These figures illustrate the model's capability to handle diverse and challenging scenarios effectively. In these examples, our model demonstrates strong performance in object-level reasoning tasks, highlighting EventGPT’s ability to reason complex visual information within the scene.

% In Figure~\ref{fig: object-detection}, EventGPT demonstrates remarkable accuracy in detecting objects across different environments, including low-light conditions and scenarios with fast-moving objects. This highlights the model's robustness in handling temporal dynamics, a feature attributed to its event-based architecture

% Similarly, Figure~\ref{fig: object-segmentation} showcases EventGPT's proficiency in instance segmentation, where it accurately delineates object boundaries even in complex scenes with occlusions. The model's ability to maintain high precision in such scenarios underscores its potential for real-world applications in autonomous systems and robotics

% In conclusion, the qualitative analysis presented here reinforces the robustness of EventGPT in handling diverse downstream tasks. Future work will explore quantitative evaluations and comparisons with baseline models to further validate these findings.
